# Supplementary material for: Well-rounded sublattices of planar lattices
Source: arXiv:1311.6306 source file (2014-09-04)
Supplement: Supplementary file 1 [file supplement-final.pdf]

# SUPPLEMENT TO "WELL-ROUNDED SUBLATTICES OF PLANAR LATTICES"

PETER ZEINER

Abstract. Additional material to the article "Well-rounded sublattices of planar lattices", including some calculations on the asymptotic behaviour of various arithmetic functions and some remarks on BRS lattices.

In this supplement we present the details of our calculations for the asymptotic growth rates of the number of well-rounded sublattices, which we have mentioned only briefly in our main article. In addition, we add some details on BRS lattices.

This supplement was initially intended for private use only, but it has been adapted for a wider audience now. Nevertheless, some parts are rather sketchy, and the explicit calculations vary in style, rangeing from very detailed textbook-like calculations to rather short ones.

Section numbers, equations, theorem etc. of this supplement have a prefix "Su", whereas all references to sections, equations and theorems without prefix refer to our main article (version 2 on the arXiv).

## Su-1. Explicit expressions for BRS lattices

In Section 5.1 we have discussed the existence of well-rounded lattices. In particular, Prop. 2 mentions all lattices that have well-rounded sublattices and distinguishes three cases. Here, we want to give explicit formulas for BRS lattices in all three cases.

Recall that BRS lattices correspond to basic solutions of the equation

$$ac + bdn + (ad + bc)\frac{t}{2} = 0, \tag{Su-1}$$

where '*basic*' means that $\gcd(a,b) = \gcd(c,d) = 1$. By symmetry, the number of basic solutions is a multiple of eight.

Using the same methods as in the proof of Prop. 2, we obtain the following results.

**Remark Su-1.** (1) $n, t$ rational: we write $\tau = \frac{p}{q} + \mathrm{i}\beta$ with $\beta = \sqrt{\frac{r}{s}}$. Then $z_1 = a + b\tau$ and $z_2 = q^2 s \mathrm{i}\beta z_1$ yield an integral solution with $c = -(spqa + sp^2 b + rq^2 b)$, $d = s(q^2 a + pqb)$, albeit not necessarily a basic one. If $z_1$ is primitive, we get a basic solution by dividing $z_2$ by $g := \gcd\big(spqa + sp^2 b + rq^2 b, s(q^2 a + pqb)\big)$.

(2) $t$ rational, but $n$ irrational: There are only eight basic solutions. If we write $t = 2\frac{p}{q}$ with $p, q \in \mathbb{Z}$ coprime, a basic one is $a = 1, b = 0, c = p, d = -q$.

(3) $t$ irrational, with $n = \frac{p}{q} + \frac{r}{s}t$, where $q, r, s \in \mathbb{Z}\setminus\{0\}$ and $\sqrt{\frac{r^2}{s^2} + \frac{p}{q}} \in \mathbb{Q}$. There are eight basic solutions. If we define $\frac{u}{v} := \sqrt{\frac{r^2}{s^2} + \frac{p}{q}}$ a solution is given by $a = -b(\frac{r}{s} + \frac{u}{v}), b = \frac{sv}{\gcd(sv, rv+su)}, c = -d(\frac{r}{s} - \frac{u}{v}), d = \frac{sv}{\gcd(sv, rv-su)}$.

Clearly, eight basic solutions correspond to each BRS sublattice.

We have seen that two quantities play an important role for calculating the generating functions in the case of a unique BRS sublattice, namely the index $\sigma := [\Gamma : \Gamma_R]$ of this BRS sublattice and the ratio $\kappa$ of the lengths of its orthogonal basis vectors. By means of the expressions for the BRS sublattices given above we can easily compute the values of $\sigma$ and $\kappa$ explicitly for these cases. We obtain the following result.

**Remark Su-2.** The explicit values for $\sigma$ and $\kappa$ read as follows:

(1) $n$ irrational, $t$ rational with $\frac{t}{2} = \frac{p}{q}$: we have $\sigma = q, \kappa = q\sqrt{n - t^2/4}$.

(2) $t$ irrational, with $n = \frac{p}{q} + \frac{r}{s}t$, where $q, r, s \in \mathbb{Z} \setminus \{0\}$ and $\frac{u}{v} := \sqrt{\frac{r^2}{s^2} + \frac{p}{q}} \in \mathbb{Q}$: we have

$$\sigma = \frac{2s^2uv}{\gcd(sv, rv+su)\gcd(sv, rv-su)}, \quad \kappa = \frac{\gcd(sv, rv-su)}{\gcd(sv, rv+su)} \frac{\sqrt{2rv + 2su - svt}}{\sqrt{-2rv + 2su + svt}}.$$

In the special case that $n$ is rational, i.e. $n = \frac{p^2}{q^2}$ for some $p, q \in \mathbb{Z}$ coprime, the equations above simplify considerably: $\sigma = 2pq$, $\kappa = \sqrt{\frac{2\sqrt{n}-t}{2\sqrt{n}+t}}$.

## Su-2. Asymptotic behaviour — Introduction

Here, we calculate the asymptotic behaviour of certain arithmetic functions, in particular the functions counting well-rounded sublattices. We are interested in functions such as

$$A(x) = \sum_{n \le x} a(n). \tag{Su-2}$$

The functions we are interested in are typically Dirichlet convolutions of simpler funtions. If $f * g$ denotes the Dirichlet convolution, then

$$\sum_{n\le x} (f*g)(n) = \sum_{n \le x}\sum_{d|n} f(d)g(\tfrac{n}{d}) = \sum_{m\le x}\sum_{d \le x/m} f(m)g(d) \tag{Su-3}$$

$$= \sum_{m\le\sqrt{x}}\sum_{m<d\le x/m} (f(m)g(d) + f(d)g(m)) + \sum_{m\le\sqrt{x}} f(m)g(m), \tag{Su-4}$$

where the latter may allow for better error terms. [Su-1]

We often approximate sums by integrals using the Euler-Maclaurin formula

$$\sum_{y<n\le x} f(n) = \int_y^x f(t)\,dt + \int_y^x (t - [t])f'(t)\,dt + f(x)([x] - x) - f(y)([y] - y). \tag{Su-5}$$

## Su-3. Similar Sublattices

Su-3.1. **Triangular lattice.** The Dirichlet series generating function for the number of similar and primitive similar sublattices of $\mathbb{Z}[\rho]$ are

$$\Phi_{\triangle}(s) \;=\; \zeta_{\mathbb{Q}(\rho)}(s) \;=\; L(s,\chi_{-3})\zeta(s) \;=\; \sum_{n\in\mathbb{N}} \frac{b_{\triangle}(n)}{n^s} \tag{Su-6}$$

$$\Phi_{\triangle}^{\mathsf{pr}}(s) \;=\; \frac{\zeta_{\mathbb{Q}(\rho)}(s)}{\zeta(2s)} \;=\; \frac{L(s,\chi_{-3})\zeta(s)}{\zeta(2s)} \;=\; \sum_{n\in\mathbb{N}} \frac{b_{\triangle}^{\mathsf{pr}}(n)}{n^s}, \tag{Su-7}$$

respectively. We can immediately read off that

$$b_{\triangle} = 1 * \chi_{-3} \qquad \text{and} \qquad b_{\triangle}^{\mathsf{pr}} = 1 * \chi_{-3} * \nu = b_{\triangle} * \nu, \tag{Su-8}$$

with the character

$$\chi_{-3}(n) \;=\; \begin{cases} 0, & \text{if } n \equiv 0 \bmod 3,\\ 1, & \text{if } n \equiv 1 \bmod 3,\\ -1, & \text{if } n \equiv 2 \bmod 3.\end{cases}$$

and

$$\nu(n) \;=\; \begin{cases} \mu(\sqrt{n}), & \text{if } n \text{ is a square},\\ 0, & \text{otherwise},\end{cases} \tag{Su-9}$$

where $\mu$ is the Moebius function.

Su-3.1.1. *Asymptotics of similar sublattices.* We apply Eq. (Su-4) to $b_{\triangle} = 1 * \chi_{-3}$, which gives

$$\begin{aligned} \sum_{n\le x} b_{\triangle}(n) &= \sum_{m\le\sqrt{x}} \; \sum_{m<d\le x/m} \big(\chi_{-3}(d) + \chi_{-3}(m)\big) + \sum_{m\le\sqrt{x}} \chi_{-3}(m) \\ &= \sum_{m\le\sqrt{x}} \Big(O(1) + \chi_{-3}(m)\left(\left[\frac{x}{m}\right] - m\right)\Big) + O(1) \\ &= \sum_{m\le\sqrt{x}} \Big(O(1) + \chi_{-3}(m)\left(\frac{x}{m} - m\right)\Big) + O(1) \\ &= L(1,\chi_{-3})\, x + O(\sqrt{x}) = \frac{\pi}{3\sqrt{3}}\, x + O(\sqrt{x}). \end{aligned} \tag{Su-10}$$

Su-3.1.2. *Asymptotics of primitive similar sublattices.* As $b_{\triangle}^{\mathsf{pr}} = b_{\triangle} * \nu$, we can make use of Eq. (Su-4) again.

$$\sum_{n\le x} b_{\triangle}^{\mathsf{pr}}(n) = \sum_{m\le\sqrt{x}} \; \sum_{m<d\le x/m} \big(\nu(m)\, b_{\triangle}(d) + \nu(d)\, b_{\triangle}(m)\big) + \sum_{m\le\sqrt{x}} \nu(m)\, b_{\triangle}(m) \tag{Su-11}$$

The last term only contributes to the error term since

$$\left|\sum_{m\le\sqrt{x}} \nu(m)\, b_{\triangle}(m)\right| \le \sum_{m\le\sqrt{x}} b_{\triangle}(m) = O(\sqrt{x}) \tag{Su-12}$$

by Eq. (Su-10). The first term gives

(Su-13)
$$\sum_{m\le\sqrt{x}}\ \sum_{m<d\le x/m} \nu(m)\, b_\triangle(d) = \sum_{m\le\sqrt{x}} \nu(m)\left(L(1,\chi_{-3})\left(\frac{x}{m}-m\right) + O\left(\sqrt{\frac{x}{m}}\right) + O(\sqrt{m})\right)$$
$$= \frac{L(1,\chi_{-3})}{\zeta(2)}\, x + O(x^{3/4}) = \frac{2}{\pi\sqrt{3}}\, x + O(x^{3/4}),$$

where we have made use of Eqs. (Su-51)–(Su-53). The second term yields

$$\sum_{m\le\sqrt{x}}\ \sum_{m<d\le x/m} \nu(d)\, b_\triangle(m) = \sum_{m\le\sqrt{x}} b_\triangle(m) \sum_{\sqrt{m}<\ell\le\sqrt{x/m}} \mu(\ell) \tag{Su-14}$$
$$= \sum_{m\le\sqrt{x}} b_\triangle(m)\left(O(\sqrt{m}) + O\left(\sqrt{\frac{x}{m}}\right)\right)$$
$$= O(x^{3/4}),$$

where we have used Theorem Su-6. Thus

**Lemma Su-1.**

$$\sum_{n\le x} b^{\mathsf{pr}}_\triangle(n) = \frac{2}{\pi\sqrt{3}}\, x + O(x^{3/4}). \tag{Su-15}$$

Recall that $\nu$ is the arithmetic function corresponding to $\frac{1}{\zeta(2s)}$, which is analytic at $s=1$. So one might hope that this term should not influence the asymptotics too much, in particular as $\frac{1}{\zeta(2s)}$ has an abscissa of convergence of $\sigma=\frac{1}{2}$. The fact that only the first term in Eq. (Su-11) contributes to the asymptotics supports this idea. In fact, using the simpler formula

$$\sum_{n\le x} b^{\mathsf{pr}}_\triangle(n) = \sum_{m\le x}\ \sum_{d\le x/m} \nu(m)\, b_\triangle(d)$$
$$= \sum_{m\le x} \nu(m)\left(L(1,\chi_{-3})\frac{x}{m} + O\left(\sqrt{\frac{x}{m}}\right)\right)$$
$$= L(1,\chi_{-3})\, x \sum_{m\le x} \nu(m)\frac{1}{m} + \sqrt{x}\sum_{\ell\le\sqrt{x}} \mu(\ell) O\left(\frac{1}{\ell}\right)$$
$$= \frac{L(1,\chi_{-3})}{\zeta(2)}\, x + L(1,\chi_{-3})\, x O(x^{-1/2}) + \sqrt{x}\sum_{\ell\le\sqrt{x}} O\left(\frac{1}{\ell}\right)$$
$$= \frac{L(1,\chi_{-3})}{\zeta(2)}\, x + O(\sqrt{x}\log(x)) = \frac{2}{\pi\sqrt{3}}\, x + O(\sqrt{x}\log(x))$$

gives a better result. Note that we have made use of Eq. (Su-53) here. Thus

**Theorem Su-1.** *The asymptotics of the number of similar and of primitive similar sublattices of the triangular lattice is given by*

$$\sum_{n\leq x} b_{\triangle}(n) = L(1,\chi_{-3})\,x + O(\sqrt{x}) = \frac{\pi}{3\sqrt{3}}\,x + O(\sqrt{x}) \tag{Su-16}$$

*and*

$$\sum_{n\leq x} b^{\mathsf{pr}}_{\triangle}(n) = \frac{L(1,\chi_{-3})}{\zeta(2)}\,x + O(\sqrt{x}\log(x)) = \frac{2}{\pi\sqrt{3}}\,x + O(\sqrt{x}\log(x)). \tag{Su-17}$$

Su-3.2. **Square lattice.** The Dirichlet series generating function for the number of similar and primitive similar sublattices of $\mathbb{Z}[\rho]$ are

$$\Phi_{\square}(s) \;=\; \zeta_{\mathbb{Q}(i)}(s) \;=\; L(s,\chi_{-4})\zeta(s) \;=\; \sum_{n\in\mathbb{N}} \frac{b_{\square}(n)}{n^s} \tag{Su-18}$$

$$\Phi^{\mathsf{pr}}_{\square}(s) \;=\; \frac{\zeta_{\mathbb{Q}(i)}(s)}{\zeta(2s)} \;=\; \frac{L(s,\chi_{-4})\zeta(s)}{\zeta(2s)} \;=\; \sum_{n\in\mathbb{N}} \frac{b^{\mathsf{pr}}_{\square}(n)}{n^s}, \tag{Su-19}$$

respectively. We can immediately read off that

$$b_{\square} = 1 * \chi_{-4} \qquad \text{and} \qquad b^{\mathsf{pr}}_{\square} = 1 * \chi_{-4} * \nu = b_{\square} * \nu, \tag{Su-20}$$

with the character

$$\chi_{-4}(n) \;=\; \begin{cases} 0, & \text{if } n \text{ even},\\ 1, & \text{if } n \equiv 1 \bmod 4,\\ -1, & \text{if } n \equiv 3 \bmod 4. \end{cases}$$

Su-3.2.1. *Asymptotics of similar sublattices.* We apply Eq. (Su-4) to $b_{\square} = 1*\chi_{-4}$, which gives

$$\begin{aligned} \sum_{n\leq x} b_{\square}(n) &= \sum_{m\leq\sqrt{x}} \;\sum_{m<d\leq x/m} \big(\chi_{-4}(d) + \chi_{-4}(m)\big) + \sum_{m\leq\sqrt{x}} \chi_{-4}(m) \\ &= \sum_{m\leq\sqrt{x}} \Big(O(1) + \chi_{-4}(m)\left(\left[\frac{x}{m}\right] - m\right)\Big) + O(1) \\ &= \sum_{m\leq\sqrt{x}} \Big(O(1) + \chi_{-4}(m)\left(\frac{x}{m} - m\right)\Big) + O(1) \\ &= L(1,\chi_{-4})\,x + O(\sqrt{x}) = \frac{\pi}{4}\,x + O(\sqrt{x}). \end{aligned} \tag{Su-21}$$

Su-3.2.2. *Asymptotics of primitive similar sublattices.* A calculation similar to the triangular lattice gives

$$\begin{aligned}
\sum_{n\leq x} b_{\square}^{\mathsf{pr}}(n) &= \sum_{m\leq x}\ \sum_{d\leq x/m} \nu(m)\, b_{\square}(d) \\
&= \sum_{m\leq x} \nu(m) \left( L(1,\chi_{-4}) \frac{x}{m} + O\left(\sqrt{\frac{x}{m}}\right)\right) \\
&= L(1,\chi_4)\, x \sum_{m\leq x} \nu(m) \frac{1}{m} + \sqrt{x} \sum_{\ell\leq\sqrt{x}} \mu(\ell) O\left(\frac{1}{\ell}\right) \\
&= \frac{L(1,\chi_{-4})}{\zeta(2)}\, x + L(1,\chi_{-4})\, x O(x^{-1/2}) + \sqrt{x} \sum_{\ell\leq\sqrt{x}} O\left(\frac{1}{\ell}\right) \\
&= \frac{L(1,\chi_{-4})}{\zeta(2)}\, x + O(\sqrt{x}\log(x)) = \frac{3}{2\pi}\, x + O(\sqrt{x}\log(x)),
\end{aligned}$$

where we have made use of Eq. (Su-53). Thus we have proved

**Theorem Su-2.** *The asymptotics of the number of similar and of primitive similar sublattices of the square lattice is given by*

$$\sum_{n\leq x} b_{\square}(n) = L(1,\chi_{-4})\, x + O(\sqrt{x}) = \frac{\pi}{4}\, x + O(\sqrt{x}) \tag{Su-22}$$

*and*

$$\sum_{n\leq x} b_{\square}^{\mathsf{pr}}(n) = \frac{L(1,\chi_{-4})}{\zeta(2)}\, x + O(\sqrt{x}\log(x)) = \frac{3}{2\pi}\, x + O(\sqrt{x}\log(x)). \tag{Su-23}$$

## Su-4. Well-rounded sublattices

Su-4.1. **Triangular lattice.** In order to compute the number of well-rounded lattices we need the following functions

$$\sum_{n\in\mathbb{N}} \frac{w_{\triangle,even}(n)}{n^s} = \frac{1}{4^s} \sum_{p\in\mathbb{N}}\ \sum_{p<q<3p} \frac{1}{p^s q^s} \tag{Su-24}$$

$$\sum_{n\in\mathbb{N}} \frac{w_{\triangle,odd}(n)}{n^s} = \sum_{k\in\mathbb{N}}\ \sum_{k<\ell<3k+1} \frac{1}{(2k+1)^s(2\ell+1)^s} \tag{Su-25}$$

For $w_{\triangle,even}$ observe that $4pq \leq x$ together with $p < q$ means $p < \frac{\sqrt{x}}{2}$. Thus

(Su-26)

$$\begin{aligned}
\sum_{n\leq x} w_{\triangle,even}(n) &= \sum_{p<\sqrt{x}/2} \sum_{p<q\leq \min(3p-1,[x/(4p)])} 1 \\
&= \sum_{p<\sqrt{x}/2} \left(\min\left(3p-1, \left[\frac{x}{4p}\right]\right) - p\right) \\
&= \sum_{p\leq(1+\sqrt{1+3x})/6} (2p-1) + \sum_{(1+\sqrt{1+3x})/6<p<\sqrt{x}/2} \left(\left[\frac{x}{4p}\right] - p\right) \\
&= \left[\frac{1+\sqrt{1+3x}}{6}\right]^2 + \sum_{(1+\sqrt{1+3x})/6<p\leq\sqrt{x}/2} \left(\frac{x}{4p} - p + O(1)\right) \\
&= \frac{x}{12} + \frac{x}{4}\left(\log\left(\frac{\sqrt{x}}{2}\right) - \log\left(\frac{1+\sqrt{1+3x}}{6}\right)\right) - \frac{1}{2}\left(\frac{x}{4} - \frac{(1+\sqrt{1+3x})^2}{36}\right) + O(\sqrt{x}) \\
&= \frac{x}{8}\log(3) + O(\sqrt{x}).
\end{aligned}$$

Similarly we get for the odd indices — observe that $(2k+1)(2\ell+1) \leq x$ together with $k < \ell$ implies $k < \frac{\sqrt{x}-1}{2}$ —

(Su-27)
$$\begin{aligned}
\sum_{n\leq x} w_{\triangle,odd}(n) &= \sum_{k<(\sqrt{x}-1)/2} \sum_{k<\ell\leq\min(3k,[x/(4k+2)-1/2])} 1 \\
&= \sum_{k<(\sqrt{x}-1)/2} \left(\min\left(3k, \left[\frac{x}{4k+2} - \frac{1}{2}\right]\right) - k\right) \\
&= \sum_{k\leq(-1+\sqrt{4+3x})/6} 2k + \sum_{(-1+\sqrt{4+3x})/6<k<(\sqrt{x}-1)/2} \left(\left[\frac{x}{4k+2} - \frac{1}{2}\right] - k\right) \\
&= \frac{x}{12} + \frac{x}{4}\left(\log\left(\frac{\sqrt{x}}{2}\right) - \log\left(\frac{-1+\sqrt{4+3x}}{6}\right)\right) \\
&\quad - \frac{1}{2}\left(\frac{(\sqrt{x}-1)^2}{4} - \frac{(-1+\sqrt{4+3x})^2}{36}\right) + O(\sqrt{x}) \\
&= \frac{x}{8}\log(3) + O(\sqrt{x}).
\end{aligned}$$

In total, this gives for $w_{\triangle} := w_{\triangle,even} + w_{\triangle,odd}$

(Su-28)
$$\sum_{n\leq x} w_{\triangle}(n) = \frac{x}{4}\log(3) + O(\sqrt{x}).$$

The next step is to calculate

$$\sum_{n\leq x} w_{\triangle} * b_{\triangle}(n) = \sum_{m\leq\sqrt{x}} \sum_{m<d\leq x/m} \big(w_{\triangle}(m)\, b_{\triangle}(d) + w_{\triangle}(d)\, b_{\triangle}(m)\big) + \sum_{m\leq\sqrt{x}} w_{\triangle}(m)\, b_{\triangle}(m)$$

Note that both $w_\triangle$ and $b_\triangle$ are non-negative, so we can apply the asymptotic formulas for $w_\triangle$ and $b_\triangle$ also to the error terms. The first term gives

$$\begin{aligned}
&\sum_{m\le\sqrt{x}}\ \sum_{m<d\le x/m} w_\triangle(m)\, b_\triangle(d)\\
&\qquad = \sum_{m\le\sqrt{x}} w_\triangle(m)\left(L(1,\chi_{-3})\frac{x}{m}+O\left(\sqrt{\frac{x}{m}}\right)-L(1,\chi_{-3})\,m+O(\sqrt{m})\right)\\
&\qquad = L(1,\chi_{-3})x\left(\frac{\log(3)}{8}\log(x)+c_3\right)-L(1,\chi_{-3})\frac{\log(3)}{8}x+O(x^{3/4}\log(x)),\\
&\qquad = L(1,\chi_{-3})x\left(\frac{\log(3)}{8}\log(x)+c_3-\frac{\log(3)}{8}\right)+O(x^{3/4}\log(x)),
\end{aligned}$$

where we have used Eq. (Su-16) and Thm. Su-7. The second term yields

$$\begin{aligned}
&\sum_{m\le\sqrt{x}}\ \sum_{m<d\le x/m} w_\triangle(d)\, b_\triangle(m)\\
&\qquad = \sum_{m\le\sqrt{x}} b_\triangle(m)\left(\frac{x}{4m}\log(3)+O\left(\sqrt{\frac{x}{m}}\right)-\frac{m}{4}\log(3)+O(\sqrt{m})\right)\\
&\qquad = \frac{\log(3)}{4}x\left(\frac{1}{2}L(1,\chi_{-3})\log(x)+C_\triangle(1)+O(x^{-1/4}\log(x))\right)\\
&\qquad\qquad -\frac{\log(3)}{4}\left(\frac{L(1,\chi_{-3})}{2}x+O(x^{3/4})\right)\\
&\qquad = \frac{\log(3)}{8}x\left(L(1,\chi_{-3})\log(x)-L(1,\chi_{-3})+2C_\triangle(1)\right)+O(x^{3/4}\log(x)),
\end{aligned}$$

where we have used Eq. (Su-28) and Thm. Su-6. The third term only contributes to the error term. Note that $w_\triangle(m)\le d(m)$, where $d(m)$ is the divisor function. As $d(m)=o(m^\varepsilon)$ for all $\varepsilon>0$ (see [Su-1, p.296]) we see

$$\text{(Su-29)}\qquad \sum_{m\le\sqrt{x}} w_\triangle(m)\, b_\triangle(m)=\sum_{m\le\sqrt{x}} b_\triangle(m)o(m^\varepsilon)=O(x^{(1+\varepsilon)/2}).$$

Hence we get in total

$$\begin{aligned}
\sum_{n\le x} w_\triangle * b_\triangle(n) &= \frac{\log(3)}{4}L(1,\chi_{-3})x(\log(x)-1)\\
&\qquad + x\left(\frac{\log(3)}{4}C_\triangle(1)+L(1,\chi_{-3})c_3\right)+O(x^{3/4}\log(x)).
\end{aligned}$$

Taking the convolution with $\nu$ gives

$$\begin{aligned}\sum_{n\le x} w_{\triangle} * b^{\mathsf{pr}}_{\triangle}(n) &= \sum_{n\le x} \nu * w_{\triangle} * b_{\triangle}(n)\\ &= \sum_{m\le x}\sum_{d\le x/m} \nu(m)(w_{\triangle} * b_{\triangle})(d)\\ &= \sum_{m\le x}\nu(m)\Bigg(\frac{\log(3)}{4}L(1,\chi_{-3})\frac{x}{m}(\log(x)-\log(m)-1)\\ &\qquad + \frac{x}{m}\left(\frac{\log(3)}{4}C_{\triangle}(1) + L(1,\chi_{-3})c_3\right) + O\left(\frac{x^{3/4}}{m^{3/4}}\log(x/m)\right)\Bigg)\\ &= \frac{\log(3)}{4}\frac{L(1,\chi_{-3})}{\zeta(2)}x(\log(x)-1)\\ &\qquad + x\left(-\frac{\log(3)}{2}\frac{L(1,\chi_{-3})\zeta'(2)}{\zeta(2)^2} + \frac{\log(3)}{4\zeta(2)}C_{\triangle}(1) + \frac{L(1,\chi_{-3})}{\zeta(2)}c_3\right)\\ &\qquad + O(x^{3/4}\log(x)),\end{aligned}$$

where we have made use of Eqs. (Su-53) and (Su-54). Note that this has added an overall factor of $\frac{1}{\zeta(2)}$ and an addtional linear term.

Now it remains to take the factor $\frac{3}{1+3^{-s}}$ into account and add the similar sublattices. Using Lemma Su-2, we get

**Theorem Su-3.** *Let $a_{\triangle}(n)$ be the number of well-rounded sublattices of the triangular lattice with index $n$. Then, the summatory function $A_{\triangle}(x) = \sum_{n\le x} a_{\triangle}(n)$ possesses the asymptotic growth behaviour*

$$\begin{aligned}A_{\triangle}(x) &= \frac{9\log(3)}{16}\frac{L(1,\chi_{-3})}{\zeta(2)}x(\log(x)-1) + c_{\triangle}x + O(x^{3/4}\log(x))\\ &= \frac{3\sqrt{3}\log(3)}{8\pi}x(\log(x)-1) + c_{\triangle}x + O(x^{3/4}\log(x))\end{aligned} \tag{Su-30}$$

*where*

$$\begin{aligned}c_{\triangle} :=&\ \frac{9\log(3)}{16\zeta(2)}C_{\triangle}(1) + \frac{9L(1,\chi_{-3})}{4\zeta(2)}c_3 - \frac{9\log(3)}{8}\frac{L(1,\chi_{-3})\zeta'(2)}{\zeta(2)^2}\\ &+ \frac{9\log(3)^2}{64}\frac{L(1,\chi_{-3})}{\zeta(2)} + L(1,\chi_{-3})\\ =&\ L(1,\chi_{-3}) + \frac{9\log(3)L(1,\chi_{-3})}{16\zeta(2)}\Bigg(\left(\gamma + \frac{L'(1,\chi_{-3})}{L(1,\chi_{-3})} - 2\frac{\zeta'(2)}{\zeta(2)}\right) + 2\gamma - \frac{\log(3)}{4}\\ &+ \sum_{p=1}^{\infty}\frac{1}{p}\Bigg(\sum_{p<q\le 3p-1}\frac{1}{q} - \log(3)\Bigg) + \sum_{k=0}^{\infty}\frac{4}{2k+1}\Bigg(\sum_{k<\ell\le 3k}\frac{1}{2\ell+1} - \frac{1}{2}\log(3)\Bigg)\Bigg)\\ \approx&\ 0.4915036\end{aligned} \tag{Su-31}$$

*is the coefficient of* $(s-1)^{-1}$ *in the Laurent series of* $\sum_n \frac{a_\triangle(n)}{n^s}$ *around* $s=1$ *with* $C_\triangle(1)$ *and* $c_3$ *from Eqs.* (Su-62) *and* (Su-68)*, respectively.*

Su-4.2. **Square lattice.** In order to compute the number of well-rounded lattices of the square lattice we need the following functions

(Su-32)
$$\sum_{n\in\mathbb{N}} \frac{w_{\Box,even}(n)}{n^s} = \frac{1}{2^s}\sum_{p\in\mathbb{N}}\sum_{p<q<\sqrt{3}p}\frac{1}{p^s q^s}$$

(Su-33)
$$\sum_{n\in\mathbb{N}} \frac{w_{\Box,odd}(n)}{n^s} = \sum_{k\in\mathbb{N}}\sum_{k<\ell<\sqrt{3}k+(\sqrt{3}-1)/2}\frac{1}{(2k+1)^s(2\ell+1)^s}$$

(Su-34)
$$\sum_{n\in\mathbb{N}} \frac{w_{\Box,odd,2}(n)}{n^s} = \frac{1}{1+2^{-s}}\sum_{k\in\mathbb{N}}\sum_{k<\ell<\sqrt{3}k+(\sqrt{3}-1)/2}\frac{1}{(2k+1)^s(2\ell+1)^s}$$

Obviously $w_{\Box,odd,2} = g_2 * w_{\Box,odd}$, where

$$g_2(n) = \begin{cases} (-1)^r & \text{if } n = 2^r \\ 0 & \text{otherwise.} \end{cases}$$

For $w_{\Box,even}$ observe that $2pq \le x$ together with $p<q$ means $p<\sqrt{x/2}$. Thus

(Su-35)
$$\begin{aligned}
\sum_{n\le x} w_{\Box,even}(n) &= \sum_{p<\sqrt{x/2}}\ \sum_{p<q\le\min([p\sqrt{3}],[x/(2p)])} 1 \\
&= \sum_{p<\sqrt{x/2}}\left(\min\left([p\sqrt{3}],\left[\frac{x}{2p}\right]\right)-p\right) \\
&= \sum_{p\le\sqrt{x/(2\sqrt{3})}}([p\sqrt{3}]-p) + \sum_{\sqrt{x/(2\sqrt{3})}<p<\sqrt{x/2}}\left(\left[\frac{x}{2p}\right]-p\right) \\
&= \sum_{p\le\sqrt{x/(2\sqrt{3})}}(p(\sqrt{3}-1)+O(1)) + \sum_{\sqrt{x/(2\sqrt{3})}<p<\sqrt{x/2}}\left(\frac{x}{2p}-p+O(1)\right) \\
&= \frac{\sqrt{3}-1}{4\sqrt{3}}x + \frac{x}{2}\left(\log\left(\sqrt{\frac{x}{2}}\right)-\log\left(\sqrt{\frac{x}{2\sqrt{3}}}\right)\right) - \frac{1}{2}\left(\frac{x}{2}-\frac{x}{2\sqrt{3}}\right) + O(\sqrt{x}) \\
&= \frac{x}{8}\log(3) + O(\sqrt{x}).
\end{aligned}$$

Similarly, we get for the odd indices — observe that $(2k+1)(2\ell+1)\le x$ together with $k<\ell$ implies $k<\frac{\sqrt{x}-1}{2}$ —

(Su-36)
$$\sum_{n\le x} w_{\Box,odd}(n) = \sum_{k<(\sqrt{x}-1)/2}\ \sum_{k<\ell\le\min([\sqrt{3}k+(\sqrt{3}-1)/2],[x/(4k+2)-1/2])} 1$$

$$
\begin{aligned}
&= \sum_{k<(\sqrt{x}-1)/2} \left( \min\left( \left[ \sqrt{3}k + \frac{\sqrt{3}-1}{2} \right], \left[ \frac{x}{4k+2} - \frac{1}{2} \right] \right) - k \right) \\
&= \sum_{k \le \sqrt{x}/(2\sqrt[4]{3})-1/2} \left[ \sqrt{3}k + \frac{\sqrt{3}-1}{2} \right] \\
&\qquad + \sum_{(\sqrt{x}/(2\sqrt[4]{3})-1/2<k<(\sqrt{x}-1)/2} \left[ \frac{x}{4k+2} - \frac{1}{2} \right] - \sum_{k<(\sqrt{x}-1)/2} k \\
&= \frac{x}{8} + \frac{x}{4} \left( \log\left( \frac{\sqrt{x}}{2} \right) - \log\left( \frac{\sqrt{x}}{2\sqrt[4]{3}} \right) \right) - \frac{x}{8} + O(\sqrt{x}) \\
&= \frac{x}{16} \log(3) + O(\sqrt{x}).
\end{aligned}
$$

The next step is to calculate

$$
\sum_{n \le x} w_{\Box,i} * b_{\Box}(n) = \sum_{m \le \sqrt{x}} \sum_{m<d\le x/m} \big( w_{\Box,i}(m)\, b_{\Box}(d) + w_{\Box,i}(d)\, b_{\Box}(m) \big) + \sum_{m \le \sqrt{x}} w_{\Box,i}(m)\, b_{\Box}(m)
$$

for $i \in \{even, odd\}$. Note that both $w_{\Box,i}$ and $b_{\Box}$ are non-negative, so we can apply the asymptotic formulas for $w_{\Box,i}$ and $b_{\Box}$ also to the error terms. The first term gives

$$
\begin{aligned}
&\sum_{m \le \sqrt{x}} \sum_{m<d\le x/m} w_{\Box,even}(m)\, b_{\Box}(d) \\
&\quad = \sum_{m \le \sqrt{x}} w_{\Box,even}(m) \left( L(1,\chi_{-4}) \frac{x}{m} + O\left( \sqrt{\frac{x}{m}} \right) - L(1,\chi_{-4})\, m + O(\sqrt{m}) \right) \\
&\quad = L(1,\chi_{-4}) x \left( \frac{\log(3)}{16} \log(x) + c_{even} \right) - L(1,\chi_{-4}) \frac{\log(3)}{16} x + O(x^{3/4}\log(x)), \\
&\quad = L(1,\chi_{-4}) x \left( \frac{\log(3)}{16} \log(x) + c_{even} - \frac{\log(3)}{16} \right) + O(x^{3/4}\log(x)),
\end{aligned}
$$

where we have used Eq. (Su-22) and Thm. Su-9. The second term yields

$$
\begin{aligned}
&\sum_{m \le \sqrt{x}} \sum_{m<d\le x/m} w_{\Box,even}(d)\, b_{\Box}(m) \\
&\quad = \sum_{m \le \sqrt{x}} b_{\Box}(m) \left( \frac{x}{8m} \log(3) + O\left( \sqrt{\frac{x}{m}} \right) - \frac{m}{8} \log(3) + O(\sqrt{m}) \right) \\
&\quad = \frac{\log(3)}{8} x \left( \frac{1}{2} L(1,\chi_{-4}) \log(x) + C_{\Box}(1) + O(x^{-1/4}\log(x)) \right) \\
&\qquad - \frac{\log(3)}{8} \left( \frac{L(1,\chi_{-4})}{2} x + O(x^{3/4}) \right) \\
&\quad = \frac{\log(3)}{16} x \big( L(1,\chi_{-3}) \log(x) - L(1,\chi_{-3}) + 2C_{\Box}(1) \big) + O(x^{3/4}\log(x)),
\end{aligned}
$$

where we have used Eq. (Su-35) and Thm. Su-8. The third term only contributes to the error term

$$\sum_{m\le\sqrt{x}} w_{\Box,even}(m)\, b_{\Box}(m) = \sum_{m\le\sqrt{x}} b_{\Box}(m) o(m^{\varepsilon}) = O(x^{(1+\varepsilon)/2}), \tag{Su-37}$$

which is shown by the same argument as in the triangular case. Hence we get in total

$$\begin{aligned}\sum_{n\le x} w_{\Box,even} * b_{\Box}(n) &= \frac{\log(3)}{8} L(1,\chi_{-4}) x(\log(x)-1) \\ &\quad + x\left(\frac{\log(3)}{8} C_{\Box}(1) + L(1,\chi_{-4}) c_{even}\right) + O(x^{3/4}\log(x)).\end{aligned}$$

Along the same lines we get

$$\begin{aligned}\sum_{n\le x} w_{\Box,odd} * b_{\Box}(n) &= \frac{\log(3)}{16} L(1,\chi_{-4}) x(\log(x)-1) \\ &\quad + x\left(\frac{\log(3)}{16} C_{\Box}(1) + L(1,\chi_{-4}) c_{odd}\right) + O(x^{3/4}\log(x)).\end{aligned}$$

Applying Lemma Su-2 we get

$$\begin{aligned}\sum_{n\le x} w_{\Box,odd,2} * b_{\Box}(n) &= \frac{\log(3)}{24} L(1,\chi_{-4}) x(\log(x)-1) \\ &\quad + x\left(\frac{\log(3)}{24} C_{\Box}(1) + \frac{2}{3} L(1,\chi_{-4}) c_{odd} + \frac{\log(2)\log(3)}{72} L(1,\chi_{-4})\right) + O(x^{3/4}\log(x)).\end{aligned}$$

Hence we get for $w_{\Box} := w_{\Box,even} + w_{\Box,odd,2}$ the asymptotic behaviour

$$\begin{aligned}\sum_{n\le x} w_{\Box} * b_{\Box}(n) &= \frac{\log(3)}{6} L(1,\chi_{-4}) x(\log(x)-1) \\ &\quad + x\left(\frac{\log(3)}{6} C_{\Box}(1) + L(1,\chi_{-4}) c\right) + O(x^{3/4}\log(x)),\end{aligned}$$

where

$$\begin{aligned} c &= c_{even} + \frac{2}{3} c_{odd} + \frac{\log(2)\log(3)}{72} \\ &= \frac{\log(3)}{3}\left(\gamma - \frac{\log(3)}{8} - \frac{\log(2)}{12}\right) + \sum_{p=1}^{\infty} \frac{1}{2p}\left(\sum_{p<q<p\sqrt{3}} \frac{1}{q} - \frac{\log(3)}{2}\right) \\ &\quad + \frac{2}{3}\sum_{k=0}^{\infty} \frac{1}{2k+1}\left(\sum_{k<\ell<k\sqrt{3}+(\sqrt{3}-1)/2} \frac{1}{2\ell+1} - \frac{1}{4}\log(3)\right) \\ &\approx -0.5250229. \end{aligned} \tag{Su-38}$$

Taking the convolution with $\nu$ gives

$$\begin{aligned}
\sum_{n\leq x} w_\square * b_\square^{\mathsf{pr}}(n) &= \sum_{n\leq x} \nu * w_\square * b_\square(n) \\
&= \sum_{m\leq x} \sum_{d\leq x/m} \nu(m)(w_\square * b_\square)(d) \\
&= \sum_{m\leq x} \nu(m)\Bigg(\frac{\log(3)}{6} L(1,\chi_{-4})\frac{x}{m}(\log(x)-\log(m)-1) \\
&\qquad + \frac{x}{m}\left(\frac{\log(3)}{6}C_\square(1) + L(1,\chi_{-4})c\right) + O\left(\frac{x^{3/4}}{m^{3/4}}\log(x/m)\right)\Bigg) \\
&= \frac{\log(3)}{6}\frac{L(1,\chi_{-4})}{\zeta(2)} x(\log(x)-1) \\
&\qquad + x\left(-\frac{\log(3)}{3}\frac{L(1,\chi_{-3})\zeta'(2)}{\zeta(2)^2} + \frac{\log(3)}{6\zeta(2)}C_\square(1) + \frac{L(1,\chi_{-4})}{\zeta(2)}c\right) \\
&\qquad + O(x^{3/4}\log(x)),
\end{aligned}$$

Finally, multiplying by a factor 2 and adding the similar sublattices yields

**Theorem Su-4.** *Let $a_\square(n)$ be the number of well-rounded sublattices of the square lattice with index $n$. Then, the summatory function $A_\square(x) = \sum_{n\leq x} a_\square(n)$ possesses the asymptotic growth behaviour*

$$\begin{aligned}
A_\square(x) &= \frac{\log(3)}{3}\frac{L(1,\chi_{-4})}{\zeta(2)} x(\log(x)-1) + c_\square x + O(x^{3/4}\log(x)) \\
&= \frac{\log(3)}{2\pi} x(\log(x)-1) + c_\square x + O(x^{3/4}\log(x))
\end{aligned} \tag{Su-39}$$

*where*

(Su-40)

$$\begin{aligned}
c_\square &:= \frac{\log(3)}{3\zeta(2)}C_\square(1) + \frac{2L(1,\chi_{-4})}{\zeta(2)}c - \frac{2\log(3)}{3}\frac{L(1,\chi_{-4})\zeta'(2)}{\zeta(2)^2} + L(1,\chi_{-4}) \\
&= \frac{L(1,\chi_{-4})}{\zeta(2)}\Bigg(\zeta(2) + \frac{\log(3)}{3}\left(\frac{L'(1,\chi_{-4})}{L(1,\chi_{-4})} + \gamma - 2\frac{\zeta'(2)}{\zeta(2)}\right) + \frac{\log(3)}{3}\left(2\gamma - \frac{\log(3)}{4} - \frac{\log(2)}{6}\right) \\
&\qquad + \sum_{p=1}^{\infty}\frac{1}{p}\left(\sum_{p<q<p\sqrt{3}}\frac{1}{q} - \frac{\log(3)}{2}\right) \\
&\qquad + \frac{4}{3}\sum_{k=0}^{\infty}\frac{1}{2k+1}\left(\sum_{k<\ell<k\sqrt{3}+(\sqrt{3}-1)/2}\frac{1}{2\ell+1} - \frac{1}{4}\log(3)\right)\Bigg) \\
&\approx 0.6272237
\end{aligned}$$

*is the coefficient of* $(s-1)^{-1}$ *in the Laurent series of* $\sum_n \frac{a_\Box(n)}{n^s}$ *around* $s=1$ *with* $C_\Box(1)$ *and* $c$ *from Eqs.* (Su-75) *and* (Su-38), *respectively.*

Su-4.3. **Lattices with exactly one BRS lattice (i.e., lattices with exactly one non-trivial CSL).** In this case we need

$$\phi_{\mathsf{wr},even}(\kappa;s)=\sum_{n\in\mathbb{N}}\frac{w_{even}(\kappa,n)}{n^s}=\frac{1}{2^s}\sum_{p\in\mathbb{N}}\sum_{\frac{\kappa}{\sqrt{3}}p<q<\sqrt{3}\,\kappa\,p}\frac{1}{p^sq^s} \tag{Su-41}$$

$$\phi_{\mathsf{wr},odd}(\kappa;s)=\sum_{n\in\mathbb{N}}\frac{w_{odd}(\kappa,n)}{n^s}=\sum_{k\in\mathbb{N}}\sum_{\frac{\kappa}{\sqrt{3}}(k+\frac12)-\frac12<\ell<\sqrt{3}\,\kappa\,(k+\frac12)-\frac12}\frac{1}{(2k+1)^s(2\ell+1)^s} \tag{Su-42}$$

Here $\kappa\sqrt{3}\notin\mathbb{Q}$ and we may assume w.l.o.g. $\kappa\geq 1$. For $w_{even}$ observe that $2pq\leq x$ together with $p<\frac{q\sqrt{3}}{\kappa}$ means $p<\sqrt{\frac{x\sqrt{3}}{2\kappa}}$ and thus

$$\begin{aligned}
\sum_{n\leq x}w_{even}(\kappa,n) &= \sum_{p<\sqrt{x\sqrt{3}/(2\kappa)}}\ \sum_{p\kappa/\sqrt{3}<q\leq\min([p\sqrt{3}\,\kappa],[x/(2p)])} 1\\
&= \sum_{p<\sqrt{x/(2\kappa\sqrt{3})}}\left(\frac{2p\kappa}{\sqrt{3}}+O(1)\right)+\sum_{\sqrt{x/(2\kappa\sqrt{3})}\leq p<\sqrt{x\sqrt{3}/(2\kappa)}}\left(\frac{x}{2p}-\frac{p\kappa}{\sqrt{3}}+O(1)\right)\\
&= \frac{x}{6}+\frac{x}{2}\log\left(\frac{\sqrt{x\sqrt{3}/(2\kappa)}}{\sqrt{x/(2\kappa\sqrt{3})}}\right)-\frac{\kappa}{2\sqrt{3}}\left(\frac{x\sqrt{3}}{2\kappa}-\frac{x}{2\kappa\sqrt{3}}\right)+O(\sqrt{x})\\
&= \frac{x}{4}\log 3+O(\sqrt{x}).
\end{aligned}$$

Note that the leading term is independent of $\kappa$.

Similarly, we get for the odd indices — observe that $(2k+1)(2\ell+1)\leq x$ together with $\frac{\kappa}{\sqrt{3}}(2k+1)<2\ell+1$ implies $k<\sqrt{\frac{x\sqrt{3}}{4\kappa}}-\frac12$ —

$$\begin{aligned}
\sum_{n\leq x}w_{odd}(\kappa,n) &= \sum_{k<\sqrt{x\sqrt{3}/(4\kappa)}-1/2}\ \sum_{\frac{\kappa}{\sqrt{3}}(k+\frac12)-\frac12<\ell\leq\min([\sqrt{3}\,\kappa\,(k+\frac12)-\frac12],[\frac{x}{4k+2}-\frac12])} 1\\
&= \sum_{k<\sqrt{x/(4\kappa\sqrt{3})}-1/2}\left(\frac{\kappa(2k+1)}{\sqrt{3}}+O(1)\right)\\
&\quad+\sum_{\sqrt{x/(4\kappa\sqrt{3})}-1/2\leq k<\sqrt{x\sqrt{3}/(4\kappa)}-1/2}\left(\frac{x}{4k+2}-\frac{\kappa}{\sqrt{3}}\left(k+\frac12\right)+O(1)\right)\\
&= \frac{x}{12}+\frac{x}{4}\log\left(\frac{\sqrt{x\sqrt{3}/(4\kappa)}}{\sqrt{x/(4\kappa\sqrt{3})}}\right)-\frac{\kappa}{2\sqrt{3}}\left(\frac{x\sqrt{3}}{4\kappa}-\frac{x}{4\kappa\sqrt{3}}\right)+O(\sqrt{x})\\
&= \frac{x}{8}\log 3+O(\sqrt{x}).
\end{aligned}$$

Taking the index of the (unique) BRS sublattice into account we finally get

**Proposition Su-1.** *Let $\Gamma$ be a lattice that has a well-rounded sublattice and assume that at least one of $n$ and $t$ is irrational. Let $\sigma$ be the index of the BRS sublattice and $\kappa$ be the ratio of the lengths of its orthogonal basis vectors. Let $a_\Gamma(n)$ denote the number of well-rounded sublattices of $\Gamma$ with index $n$. Then, the summatory function $A_\Gamma(x) = \sum_{n\leq x} a_\Gamma(n)$ possesses the asymptotic growth behaviour*

$$A_\Gamma(x) = \begin{cases} \frac{\log 3}{4\sigma}x + O(\sqrt{x}) & \text{if } \sigma \text{ is odd} \\ \frac{\log 3}{2\sigma}x + O(\sqrt{x}) & \text{if } \sigma \text{ is even.} \end{cases} \tag{Su-43}$$

*In particular, the leading term is independent of $\kappa$ and depends on $\sigma$ only.*

Recall that the BRS sublattice is a CSL if and only if it has odd index (we do not have square sublattices in the present case). Hence, if $\Sigma$ is the index of the unique non-trivial CSL, then $\sigma = \Sigma$ if $\sigma$ is odd and $\sigma = 2\Sigma$ if $\sigma$ is even. Thus we can reformulate our results as follows:

**Theorem Su-5.** *Let $\Gamma$ be a lattice that has a well-rounded sublattice and assume that at least one of $n$ and $t$ is irrational, i.e. $\Gamma$ has exactly one non-trivial CSL. Let $\Sigma$ be its index in $\Gamma$. Let $a_\Gamma(n)$ denote the number of well-rounded sublattices of $\Gamma$ with index $n$. Then, the summatory function $A_\Gamma(x) = \sum_{n\leq x} a_\Gamma(n)$ possesses the asymptotic growth behaviour*

$$A_\Gamma(x) = \frac{\log 3}{4\Sigma}x + O(\sqrt{x}). \tag{Su-44}$$

## Appendix Su-A. Some formulas

Su-A.1. **General formulas.** We first cite some well-known formulas, see [Su-1, Thm. 3.2]. It is always to be understood that summation starts with $n = 1$.

$$\sum_{n\leq y} n^s = \frac{1}{s+1}\, y^{s+1} + O(y^s) \qquad \text{for } s > 0 \tag{Su-45}$$

$$\sum_{n\leq y} \frac{1}{n^s} = \frac{1}{1-s}y^{1-s} + \zeta(s) + O(y^{-s}) \qquad \text{for } s > 0, s \neq 1 \tag{Su-46}$$

$$\sum_{n\leq y} \frac{1}{n} = \log(y) + \gamma + O\left(\frac{1}{y}\right), \tag{Su-47}$$

where $\gamma \approx 0.57721566$ is the Euler-Mascheroni constant. We also need the following variant for sums over odd integers $n \geq 3$

$$\begin{aligned} \sum_{k\leq y} \frac{1}{2k+1} &= \frac{1}{2}\log(2y+1) + \frac{1}{2}\gamma + \frac{1}{2}\log(2) - 1 + O\left(\frac{1}{y}\right) \\ &= \frac{1}{2}\log(y) + \frac{1}{2}\gamma + \log(2) - 1 + O\left(\frac{1}{y}\right). \end{aligned} \tag{Su-48}$$

Furthermore, we need a formula involving the logarithm

$$\sum_{n\le y}\frac{\log(n)}{n}=\frac{1}{2}\log(y)^2+\gamma_1+O\left(\frac{\log(y)}{y}\right), \tag{Su-49}$$

where

$$\gamma_1=\lim_{n\to\infty}\sum_{k=1}^{n}\frac{\log(k)}{k}-\frac{1}{2}\log(n)^2\approx -0.07281585 \tag{Su-50}$$

is the first Stieltjes constant.

Next we state some formulas involving the Moebius function. For $s>-\frac{1}{2}$,

$$\sum_{n\le y}\nu(n)\,n^s=\sum_{m\le\sqrt{y}}\mu(m)\,m^{2s}=O(y^{s+\frac{1}{2}}) \tag{Su-51}$$

is a rough estimate, which is good enough for our purposes. This equation even holds for $s=-\frac{1}{2}$ as

$$\left|\sum_{n\le y}\nu(n)\,n^{-1/2}\right|=\left|\sum_{m\le\sqrt{y}}\mu(m)\,\frac{1}{m}\right|\le 1, \tag{Su-52}$$

see [Su-1, Thm. 3.13] for a proof. For $s<-\frac{1}{2}$

$$\sum_{n\le y}\nu(n)\,n^s=\sum_{m\in\mathbb{N}}\mu(m)\,m^{2s}-\sum_{m>\sqrt{y}}\mu(m)\,m^{2s}=\frac{1}{\zeta(-2s)}+O(y^{s+\frac{1}{2}}). \tag{Su-53}$$

In addition, we mention

(Su-54)
$$\sum_{n\le y}\nu(n)\,\frac{\log(n)}{n^s}=2\sum_{m\in\mathbb{N}}\mu(m)\,\frac{\log(m)}{m^{2s}}-2\sum_{m>\sqrt{y}}\mu(m)\,\frac{\log(m)}{m^{2s}}=2\frac{\zeta'(2s)}{\zeta(2s)^2}+O(y^{\frac{1}{2}-s}\log(y)),$$

which holds for $s>\frac{1}{2}$.

Finally we state

**Lemma Su-2.** *Let $f$ be an arithmetic function such that $\sum_{n\le x}f(n)=ax\log(x)+bx+O(x^\alpha\log(x))$ with $0<\alpha<1$ and*

$$g(n)=\begin{cases}(-1)^r & \text{if } n=q^r\\ 0 & \text{otherwise,}\end{cases}$$

*where $q$ is some fixed positive integer. Then*

$$\sum_{n\le x}f*g(n)=\frac{q}{q+1}\,(ax\log(x)+bx)+\frac{q\log(q)}{(q+1)^2}ax+O(x^\alpha\log(x)). \tag{Su-55}$$

Su-A.2. **Triangular lattice.** In the following, $k$ is always a positive integer.

Su-A.2.1. *Formulas for $\chi_{-3}$.* For $s > 0$ we have

$$\sum_{n\leq y} \chi_{-3}(n) = \left[\frac{y-1}{3}\right] - \left[\frac{y-2}{3}\right] = O(1) \tag{Su-56}$$

$$\sum_{n\leq y} \chi_{-3}(n) n^s = O(y^s) \tag{Su-57}$$

$$\sum_{n\leq y} \frac{\chi_{-3}(n)}{n^s} = \sum_{n\in\mathbb{N}} \frac{\chi_{-3}(n)}{n^s} - \sum_{y<n} \frac{\chi_{-3}(n)}{n^s} = L(s,\chi_{-3}) + O\left(\frac{1}{y^s}\right) \tag{Su-58}$$

$$\sum_{k<n\leq y} \frac{\chi_{-3}(n)}{n^s} = \sum_{k<n} \frac{\chi_{-3}(n)}{n^s} + O\left(\frac{1}{y^s}\right) = O\left(\frac{1}{k^s}\right) + O\left(\frac{1}{y^s}\right) \tag{Su-59}$$

Su-A.2.2. *Formulas involving $b_\triangle$.* For $s > 0$

$$\begin{aligned}
\sum_{n\leq y} b_\triangle(n) n^s &= \sum_{m\leq\sqrt{y}} \sum_{m<d\leq y/m} \big(\chi_{-3}(m) + \chi_{-3}(d)\big)(md)^s + \sum_{m\leq\sqrt{y}} \chi_{-3}(m) m^{2s} \\
&= \sum_{m\leq\sqrt{y}} m^s \chi_{-3}(m) \frac{1}{s+1}\left(\frac{y^{s+1}}{m^{s+1}} - m^{s+1}\right) \\
&\quad + \sum_{m\leq\sqrt{y}} m^s \left(O\left(\frac{y^s}{m^s}\right) + O(m^s)\right) + O(y^s) \\
&= \frac{1}{s+1} L(1,\chi_{-3})\, y^{s+1} + O(y^{s+\frac{1}{2}})
\end{aligned}$$

for $0 < s < \frac{1}{2}$

$$\begin{aligned}
\sum_{n\leq y} \frac{b_\triangle(n)}{n^s} &= \sum_{m\leq\sqrt{y}} \sum_{m<d\leq y/m} \frac{\chi_{-3}(m) + \chi_{-3}(d)}{(md)^s} + \sum_{m\leq\sqrt{y}} \frac{\chi_{-3}(m)}{m^{2s}} \\
&= \sum_{m\leq\sqrt{y}} \frac{\chi_{-3}(m)}{m^s} \frac{1}{1-s}\left(\frac{y^{1-s}}{m^{1-s}} - m^{1-s}\right) \\
&\quad + \sum_{m\leq\sqrt{y}} \frac{1}{m^s}\left(O\left(\frac{y^{-s}}{m^{-s}}\right) + O(m^{-s})\right) + L(2s,\chi_{-3}) + O\left(\frac{1}{y^s}\right) \\
&= \frac{L(1,\chi_{-3})}{1-s}\, y^{1-s} + O(y^{1/2-s})
\end{aligned}$$

for $\frac{1}{2} < s < 1$

$$\begin{aligned}
\sum_{n\leq y} \frac{b_\triangle(n)}{n^s} &= \sum_{m\leq\sqrt{y}} \sum_{m<d\leq y/m} \frac{\chi_{-3}(m) + \chi_{-3}(d)}{(md)^s} + \sum_{m\leq\sqrt{y}} \frac{\chi_{-3}(m)}{m^{2s}} \\
&= \sum_{m\leq\sqrt{y}} \frac{\chi_{-3}(m)}{m^s}\left(\frac{1}{1-s}\frac{y^{1-s}}{m^{1-s}} + \zeta(s) + O\left(\frac{y^{-s}}{m^{-s}}\right) - \sum_{d=1}^{m} \frac{1}{d^s}\right)
\end{aligned}$$

$$+\sum_{m\le\sqrt{y}}\frac{1}{m^s}\left(\sum_{d=m+1}^{\infty}\frac{\chi_{-3}(d)}{d^s}+O\left(\frac{m^s}{y^s}\right)\right)+L(2s,\chi_{-3})+O\left(\frac{1}{y^s}\right)$$
$$=\frac{L(1,\chi_{-3})}{1-s}\,y^{1-s}+C(s)+O(y^{1/2-s}),$$

with

$$C(s)=L(s,\chi_{-3})\zeta(s)-\sum_{m=1}^{\infty}\frac{\chi_{-3}(m)}{m^s}\sum_{d=1}^{m}\frac{1}{d^s}+\sum_{m=1}^{\infty}\frac{1}{m^s}\sum_{d=m+1}^{\infty}\frac{\chi_{-3}(d)}{d^s}+L(2s,\chi_{-3}).$$

The sums in $C(s)$ are Dirichlet series that converge for $\mathrm{Re}(s)>\frac{1}{2}$, and are thus analytic for $\mathrm{Re}(s)>\frac{1}{2}$. They converge absolutely for $\mathrm{Re}(s)>1$, and a reordering of terms shows that the last three terms add up to zero for $\mathrm{Re}(s)>1$, and hence due to the analyticity also for $\mathrm{Re}(s)>\frac{1}{2}$. Hence $C(s)=L(s,\chi_{-3})\zeta(s)$ and thus

$$\sum_{n\le y}\frac{b_{\triangle}(n)}{n^s}=\frac{L(1,\chi_{-3})}{1-s}\,y^{1-s}+L(s,\chi_{-3})\zeta(s)+O(y^{1/2-s})$$

for $\frac{1}{2}<s<1$. For $s=\frac{1}{2}$ the situation is a bit more tricky and we want to avoid logarithmic error terms. The only two difficult terms are

$$\sum_{m\le\sqrt{y}}\frac{\chi_{-3}(m)}{m^s}\sum_{d=1}^{m}\frac{1}{d^s}\qquad\text{and}\qquad\sum_{m\le\sqrt{y}}\frac{1}{m^s}\sum_{d=m+1}^{\infty}\frac{\chi_{-3}(d)}{d^s}$$

The first term

$$\sum_{m\le\sqrt{y}}\frac{\chi_{-3}(m)}{m^s}\sum_{d=1}^{m}\frac{1}{d^s}=\sum_{k\le(\sqrt{y}-1)/3}\left(\left(\frac{1}{(3k+1)^s}-\frac{1}{(3k+2)^s}\right)\sum_{d=1}^{3k+1}\frac{1}{d^s}-\frac{1}{(3k+2)^{2s}}\right)$$
$$+O\left(\frac{1}{\sqrt{y}^s}\right)\sum_{d\le\sqrt{y}}\frac{1}{d^s}$$
$$=\sum_{k\le(\sqrt{y}-1)/3}\left(\frac{1}{(3k+1)^s}\left(\frac{s}{3k+1}+O\left(\frac{1}{(3k+1)^2}\right)\right)\left(\frac{(3k+1)^{1-s}}{1-s}+O(1)\right)\right.$$
$$\left.-\frac{1}{(3k+2)^{2s}}\right)+O(y^{1/2-s})$$
$$=\left(\frac{s}{1-s}-1\right)\sum_{k\le(\sqrt{y}-1)/3}\frac{1}{(3k+1)^{2s}}$$
$$+\sum_{k\le(\sqrt{y}-1)/3}O\left(\frac{1}{(3k+1)^{s+1}}\right)+O(y^{1/2-s})$$

is seen to be bounded for $1 > s \geq \frac{1}{2}$ and so is the second term

$$\begin{aligned}
\sum_{m\leq\sqrt{y}} \frac{1}{m^s} \sum_{d=m+1}^{\infty} \frac{\chi_{-3}(d)}{d^s} &= \sum_{0\leq k\leq(\sqrt{y}-1)/3} \sum_{j=1}^{3} \frac{1}{(3k+j)^s} \sum_{d=3k+j+1}^{\infty} \frac{\chi_{-3}(d)}{d^s} + O(y^{-s}) \\
&= \sum_{0\leq k\leq(\sqrt{y}-1)/3} \left( \frac{1}{(3k+1)^s} \frac{-2}{3(3k+2)^s} + \frac{1}{(3k+2)^s} \frac{1}{3(3k+4)^s} \right. \\
&\qquad \left. + \frac{1}{(3k+3)^s} \frac{1}{3(3k+4)^s} + O\left(\frac{1}{k^{1+2s}}\right)\right) + O(y^{-s}) \\
&= \sum_{0\leq k\leq(\sqrt{y}-1)/3} O\left(\frac{1}{k^{1+2s}}\right) + O(y^{-s})
\end{aligned}$$

where we have made use of

$$\begin{aligned}
\sum_{d=3k}^{\infty} \frac{\chi_{-3}(d)}{d^s} &= \sum_{d=3k+1}^{\infty} \frac{\chi_{-3}(d)}{d^s} \\
&= \sum_{\ell=k}^{\infty} \left( \frac{1}{(3\ell+1)^s} - \frac{1}{(3\ell+2)^s} \right) \\
&= \sum_{\ell=k}^{\infty} \frac{1}{(3\ell+1)^s} \left( \frac{s}{3\ell+1} + O\left(\frac{1}{(3\ell+1)^2}\right)\right) \\
&= \frac{1}{3(3k+1)^s} + O\left(\frac{1}{k^{1+s}}\right)
\end{aligned}$$

and

$$\begin{aligned}
\sum_{d=3k+2}^{\infty} \frac{\chi_{-3}(d)}{d^s} &= -\sum_{\ell=k}^{\infty} \left( \frac{1}{(3\ell+2)^s} - \frac{1}{(3\ell+4)^s} \right) \\
&= -\frac{2}{3(3k+2)^s} + O\left(\frac{1}{k^{1+s}}\right).
\end{aligned}$$

Hence

$$\sum_{n\leq y} \frac{b_{\triangle}(n)}{n^{1/2}} = 2L(1,\chi_{-3})\, y^{1/2} + O(1).$$

For $s = 1$ we get

$$\begin{aligned}
\sum_{n\leq y} \frac{b_{\triangle}(n)}{n} &= \sum_{m\leq\sqrt{y}} \sum_{m<d\leq y/m} \frac{\chi_{-3}(m) + \chi_{-3}(d)}{md} + \sum_{m\leq\sqrt{y}} \frac{\chi_{-3}(m)}{m^2} \\
&= \sum_{m\leq\sqrt{y}} \frac{\chi_{-3}(m)}{m} \left( \log\left(\frac{y}{m}\right) + \gamma + O\left(\frac{m}{y}\right) - \sum_{d=1}^{m} \frac{1}{d} \right) \\
&\qquad + \sum_{m\leq\sqrt{y}} \frac{1}{m} \left( \sum_{d=m+1}^{\infty} \frac{\chi_{-3}(d)}{d} + O\left(\frac{m}{y}\right)\right) + L(2,\chi_{-3}) + O\left(\frac{1}{y}\right)
\end{aligned}$$

$$= L(1,\chi_{-3})\log(y) + C(1) + O(y^{-1/2}\log(y)),$$

with

$$\begin{aligned} C(1) &= L(1,\chi_{-3})\gamma - \sum_{m=1}^{\infty} \frac{\chi_{-3}(m)}{m}\left(\log(m) + \sum_{d=1}^{m}\frac{1}{d}\right) \\ &\quad + \sum_{m=1}^{\infty}\frac{1}{m}\sum_{d=m+1}^{\infty}\frac{\chi_{-3}(d)}{d} + L(2,\chi_{-3}) \\ &= L(1,\chi_{-3})\gamma - \sum_{m=1}^{\infty}\frac{\chi_{-3}(m)}{m}\log(m) = L(1,\chi_{-3})\gamma + L'(1,\chi_{-3}). \end{aligned}$$

by a similar argument as above.

For $s > 1$ we get

$$\begin{aligned} \sum_{n\le y}\frac{b_{\triangle}(n)}{n^s} &= \sum_{m\le\sqrt{y}}\ \sum_{m<d\le y/m}\frac{\chi_{-3}(m)+\chi_{-3}(d)}{(md)^s} + \sum_{m\le\sqrt{y}}\frac{\chi_{-3}(m)}{m^{2s}} \\ &= \sum_{m\le\sqrt{y}}\frac{\chi_{-3}(m)}{m^s}\left(\zeta(s) + \frac{1}{1-s}\frac{m^{s-1}}{y^{s-1}} + O\left(\frac{m^s}{y^s}\right) - \sum_{d=1}^{m}\frac{1}{d^s}\right) \\ &\quad + \sum_{m\le\sqrt{y}}\frac{1}{m^s}\left(\sum_{d=m+1}^{\infty}\frac{\chi_{-3}(d)}{d^s} + O\left(\frac{m^s}{y^s}\right)\right) + L(2s,\chi_{-3}) + O\left(\frac{1}{y^s}\right) \\ &= L(s,\chi_{-3})\zeta(s) + \frac{L(1,\chi_{-3})}{1-s}\,y^{1-s} + O(y^{-s/2}), \end{aligned}$$

where we again have used the identity

$$-\sum_{m=1}^{\infty}\frac{\chi_{-3}(m)}{m^s}\sum_{d=1}^{m}\frac{1}{d^s} + \sum_{m=1}^{\infty}\frac{1}{m^s}\sum_{d=m+1}^{\infty}\frac{\chi_{-3}(d)}{d^s} + L(2s,\chi_{-3}) = 0. \tag{Su-60}$$

Summarising we have

**Theorem Su-6.**

$$\sum_{n\le y} b_{\triangle}(n)n^{-s} = \begin{cases} \frac{L(1,\chi_{-3})}{1-s}\,y^{1-s} + O(y^{1/2-s}) & \textit{for } s<\frac{1}{2} \\ 2L(1,\chi_{-3})\,y^{1/2} + O(1) & \textit{for } s=\frac{1}{2} \\ \frac{L(1,\chi_{-3})}{1-s}\,y^{1-s} + L(s,\chi_{-3})\zeta(s) + O(y^{1/2-s}) & \textit{for } \frac{1}{2}<s<1 \\ L(1,\chi_{-3})\log(y) + C_{\triangle}(1) + O(y^{-1/2}\log(y)) & \textit{for } s=1 \\ L(s,\chi_{-3})\zeta(s) + \frac{L(1,\chi_{-3})}{1-s}\,y^{1-s} + O(y^{-s/2}) & \textit{for } s>1 \end{cases} \tag{Su-61}$$

*where*

$$C_{\triangle}(1) = L(1,\chi_{-3})\gamma + L'(1,\chi_{-3}) \approx 0.5716475. \tag{Su-62}$$

Note that $L'(1,\chi_{-3})$ can be computed efficiently (see [Su-2] and references therein), in particular

$$\text{(Su-63)}\qquad \frac{L'(1,\chi_{-3})}{L(1,\chi_{-3})} = \log\left(\frac{2^{\frac{3}{4}}M\left(1,\cos(\frac{\pi}{12})\right)^2 e^{\gamma}}{3}\right) = \log\left(\frac{2^4\pi^4 e^{\gamma}}{3^{\frac{3}{2}}\Gamma\left(\frac{1}{3}\right)^6}\right),$$

where $M(x,y)$ is the arithmetic-geometric mean of $x$ and $y$.

Su-A.2.3. *Formulas for $w_\triangle$.* For $s > -1$ we have

$$\begin{aligned}
\sum_{n\le y} w_{\triangle,even}(n)n^s &= \sum_{p<\sqrt{y}/2}\ \sum_{p<q\le\min(3p-1,[y/(4p)])} (4pq)^s \\
&= \sum_{p\le(1+\sqrt{1+3y})/6} (4p)^s \sum_{p<q\le 3p-1} q^s + \sum_{(1+\sqrt{1+3y})/6<p<\sqrt{y}/2} (4p)^s \sum_{p<q\le[y/(4p)]} q^s \\
&= \sum_{p\le(1+\sqrt{1+3y})/6} (4p)^s \left(\frac{1}{s+1}p^{1+s}(3^{s+1}-1)+O(p^s)\right) \\
&\quad + \sum_{(1+\sqrt{1+3y})/6<p<\sqrt{y}/2} (4p)^s \left(\frac{1}{s+1}\left(\frac{y^{s+1}}{(4p)^{s+1}} - p^{s+1}\right) + O(p^s) + O\left(\frac{y^s}{p^s}\right)\right) \\
&= \frac{4^s(3^{s+1}-1)}{2(s+1)^2}\frac{(3y)^{s+1}}{6^{2s+2}} + O(y^{s+\frac{1}{2}}) + O(1) \\
&\quad + \frac{y^{s+1}}{4(s+1)}\log\left(\frac{3\sqrt{y}}{1+\sqrt{1+3y}}\right) - \frac{4^s}{2(s+1)^2}\left(\frac{y^{s+1}}{2^{2s+2}} - \frac{(3y)^{s+1}}{6^{2s+2}}\right) \\
&= \frac{\log(3)}{8(s+1)}y^{s+1} + O(y^{s+\frac{1}{2}}) + O(1).
\end{aligned}$$

Similarly (again for $s > -1$)

$$\begin{aligned}
\sum_{n\le y} w_{\triangle,odd}(n)n^s &= \sum_{k<(\sqrt{y}-1)/2}\ \sum_{k<\ell\le\min(3k,[y/(4k+2)-1/2])} (2k+1)^s(2\ell+1)^s \\
&= \sum_{k\le(-1+\sqrt{4+3y})/6} (2k+1)^s \sum_{k<\ell\le 3k} (2\ell+1)^s \\
&\quad + \sum_{(-1+\sqrt{4+3y})/6<k<(\sqrt{y}-1)/2} (2k+1)^s \sum_{k<\ell\le[y/(4k+2)-1/2]} (2\ell+1)^s \\
&= \sum_{k\le(-1+\sqrt{4+3y})/6} (2k+1)^s \frac{1}{2(s+1)} \underbrace{\left((6k+1)^{s+1} - (2k+1)^{s+1}\right)}_{(3^{s+1}-1)(2k+1)^{s+1}+O(k^s)} \\
&\quad + \sum_{(-1+\sqrt{4+3y})/6<k<(\sqrt{y}-1)/2} (2k+1)^s \times \\
&\quad \times \left(\frac{1}{2(s+1)}\left(\frac{y^{s+1}}{(2k+1)^{s+1}} - (2k+1)^{s+1}\right) + O(k^s) + O\left(\frac{y^s}{(2k+1)^s}\right)\right)
\end{aligned}$$

$$
\begin{aligned}
&= \frac{3^{s+1}-1}{8(s+1)^2}\frac{2^{2s+2}(3y)^{s+1}}{6^{2s+2}} + O(y^{s+\frac{1}{2}}) + O(1) \\
&\quad + \frac{y^{s+1}}{4(s+1)}\log\left(\frac{3(\sqrt{y}-1)}{-1+\sqrt{4+3y}}\right) \\
&\quad - \frac{1}{8(s+1)^2}\left(\frac{(\sqrt{y}-1)^{2s+2}}{2^{2s+2}} - \frac{(-1+\sqrt{4+3y})^{2s+2}}{6^{2s+2}}\right) \\
&= \frac{\log(3)}{8(s+1)}y^{s+1} + O(y^{s+\frac{1}{2}}) + O(1),
\end{aligned}
$$

and hence in total for $s > -1$

$$
\sum_{n\le y} w_{\triangle}(n)n^s = \sum_{n\le y}\left(w_{\triangle,even}(n) + w_{\triangle,odd}(n)\right)n^s = \frac{\log(3)}{4(s+1)}y^{s+1} + O(y^{s+\frac{1}{2}}) + O(1).
$$

For $s = -1$ we get

$$
\begin{aligned}
\sum_{n\le y}\frac{w_{\triangle,even}(n)}{n} &= \sum_{p<\sqrt{y}/2}\ \sum_{p<q\le\min(3p-1,[y/(4p)])}\frac{1}{4pq} \\
&= \sum_{p\le(1+\sqrt{1+3y})/6}\frac{1}{4p}\sum_{p<q\le 3p-1}\frac{1}{q} + \sum_{(1+\sqrt{1+3y})/6<p<\sqrt{y}/2}\frac{1}{4p}\sum_{p<q\le[y/(4p)]}\frac{1}{q} \\
&= \sum_{p\le(1+\sqrt{1+3y})/6}\frac{1}{4p}\Bigg(\log(3) + \underbrace{\sum_{p<q\le 3p-1}\frac{1}{q} - \log(3)}_{O\left(\frac{1}{p}\right)}\Bigg) \\
&\quad + \sum_{(1+\sqrt{1+3y})/6<p<\sqrt{y}/2}\frac{1}{4p}\left(\log\left(\frac{y}{4p^2}\right) + O\left(\frac{1}{p}\right) + O\left(\frac{p}{y}\right)\right) \\
&= \frac{\log(3)}{4}\left(\log\left(\frac{1+\sqrt{1+3y}}{6}\right) + \gamma + O(y^{-1/2})\right) \\
&\quad + \underbrace{\sum_{p=1}^{\infty}\frac{1}{4p}\left(\sum_{p<q\le 3p-1}\frac{1}{q} - \log(3)\right)}_{=:\, c_1} + O(y^{-1/2}) \\
&\quad + \frac{\log(y) - 2\log(2)}{4}\log\left(\frac{3\sqrt{y}}{1+\sqrt{1+3y}}\right) \\
&\quad - \frac{1}{4}\left(\left(\log\left(\frac{\sqrt{y}}{2}\right)\right)^2 - \left(\log\left(\frac{1+\sqrt{1+3y}}{6}\right)\right)^2\right) + O(y^{-1/2}\log(y)) \\
&= \frac{\log(3)}{8}\log(y) + \frac{\log(3)}{4}\left(\gamma - \frac{1}{4}\log(3) - \log(2)\right) + c_1 + O(y^{-1/2}\log(y)).
\end{aligned}
$$

where we have made use of

$$\left(\log\left(\frac{\sqrt{y}}{2}\right)\right)^2-\left(\log\left(\frac{1+\sqrt{1+3y}}{6}\right)\right)^2=\log\left(\frac{3\sqrt{y}}{1+\sqrt{1+3y}}\right)\log\left(\frac{\sqrt{y}(1+\sqrt{1+3y})}{12}\right)$$
$$=\frac{\log(3)}{2}\left(\log(y)-\frac{1}{2}\log(3)-2\log(2)\right)+O(y^{-1/2}\log(y))$$

Similarly

$$\begin{aligned}\sum_{n\le y}\frac{w_{\triangle,odd}(n)}{n}&=\sum_{k<(\sqrt{y}-1)/2}\ \sum_{k<\ell\le\min(3k,[y/(4k+2)-1/2])}\frac{1}{(2k+1)(2\ell+1)}\\
&=\sum_{k\le(-1+\sqrt{4+3y})/6}\frac{1}{2k+1}\sum_{k<\ell\le 3k}\frac{1}{2\ell+1}\\
&\quad+\sum_{(-1+\sqrt{4+3y})/6<k<(\sqrt{y}-1)/2}\frac{1}{2k+1}\sum_{k<\ell\le[y/(4k+2)-1/2]}\frac{1}{2\ell+1}\\
&=\sum_{k\le(-1+\sqrt{4+3y})/6}\frac{1}{2k+1}\Bigg(\frac{1}{2}\log(3)+\underbrace{\sum_{k<\ell\le 3k}\frac{1}{2\ell+1}-\frac{1}{2}\log(3)}_{O\left(\frac{1}{k}\right)}\Bigg)\\
&\quad+\sum_{(-1+\sqrt{4+3y})/6<k<(\sqrt{y}-1)/2}\frac{1}{2k+1}\left(\frac{1}{2}\log\left(\frac{y}{(2k+1)^2}\right)+O\left(\frac{1}{k}\right)+O\left(\frac{k}{y}\right)\right)\\
&=\frac{1}{2}\log(3)\left(\frac{1}{2}\log\left(\frac{-1+\sqrt{4+3y}}{6}\right)+\frac{1}{2}\gamma+\log(2)-1+O(y^{-1/2})\right)\\
&\quad+\underbrace{\sum_{k=1}^{\infty}\frac{1}{2k+1}\left(\sum_{k<\ell\le 3k}\frac{1}{2\ell+1}-\frac{1}{2}\log(3)\right)}_{=:\,c_2+\frac{1}{2}\log(3)}+O(y^{-1/2})\\
&\quad+\frac{\log(y)}{4}\log\left(\frac{3\sqrt{y}}{2+\sqrt{4+3y}}\right)\\
&\quad-\frac{1}{4}\left((\log(\sqrt{y}))^2-\left(\log\left(\frac{2+\sqrt{4+3y}}{3}\right)\right)^2\right)+O(y^{-1/2}\log(y))\\
&=\frac{\log(3)}{8}\log(y)+\frac{\log(3)}{4}\left(\gamma-\frac{1}{4}\log(3)+\log(2)\right)+c_2+O(y^{-1/2}\log(y))\end{aligned}$$

where we have made use of

$$(\log(\sqrt{y}))^2-\left(\log\left(\frac{2+\sqrt{4+3y}}{3}\right)\right)^2=\log\left(\frac{3\sqrt{y}}{2+\sqrt{4+3y}}\right)\log\left(\frac{\sqrt{y}(2+\sqrt{4+3y})}{3}\right)$$
$$=\frac{\log(3)}{2}\left(\log(y)-\frac{1}{2}\log(3)\right)+O(y^{-1/2}\log(y)).$$

In total, this gives

$$\sum_{n\le y}\frac{w_\triangle(n)}{n}=\sum_{n\le y}\frac{w_{\triangle,even}(n)+w_{\triangle,odd}(n)}{n}$$
$$=\frac{\log(3)}{4}\log(y)+\frac{\log(3)}{2}\left(\gamma-\frac{1}{4}\log(3)\right)+c_1+c_2+O(y^{-1/2}\log(y)),$$

where

$$c_1=\sum_{p=1}^{\infty}\frac{1}{4p}\left(\sum_{p<q\le 3p-1}\frac{1}{q}-\log(3)\right)\approx -0.2534695 \tag{Su-64}$$

$$c_2=\sum_{k=0}^{\infty}\frac{1}{2k+1}\left(\sum_{k<\ell\le 3k}\frac{1}{2\ell+1}-\frac{1}{2}\log(3)\right)\approx -0.6976870 \tag{Su-65}$$

Summarising we have

**Theorem Su-7.**

$$\sum_{n\le y}w_\triangle(n)n^s=\frac{\log(3)}{4(s+1)}y^{s+1}+O(y^{s+\frac{1}{2}})+O(1).\quad \textit{for } s>-1 \tag{Su-66}$$

$$\sum_{n\le y}\frac{w_\triangle(n)}{n}=\frac{\log(3)}{4}\log(y)+c_3+O(y^{-1/2}\log(y)), \tag{Su-67}$$

*where*

$$c_3:=\frac{\log(3)}{2}\left(\gamma-\frac{1}{4}\log(3)\right)+c_1+c_2\approx -0.7849570 \tag{Su-68}$$

*and $c_1$ and $c_2$ are given by Eqs.* (Su-64) *and* (Su-65)*, respectively.*

Su-A.3. **Square lattice.** In the following, $k$ is always a positive integer.

Su-A.3.1. *Formulas for $\chi_{-4}$.* For $s>0$ we have

$$\sum_{n\le y}\chi_{-4}(n)=\left[\frac{y-1}{4}\right]-\left[\frac{y-3}{4}\right]=O(1) \tag{Su-69}$$

$$\sum_{n\le y}\chi_{-4}(n)n^s=O(y^s) \tag{Su-70}$$

$$\sum_{n\le y}\frac{\chi_{-4}(n)}{n^s}=\sum_{n\in\mathbb{N}}\frac{\chi_{-4}(n)}{n^s}-\sum_{y<n}\frac{\chi_{-4}(n)}{n^s}=L(s,\chi_{-4})+O\left(\frac{1}{y^s}\right) \tag{Su-71}$$

$$\sum_{k<n\le y}\frac{\chi_{-4}(n)}{n^s}=\sum_{k<n}\frac{\chi_{-4}(n)}{n^s}+O\left(\frac{1}{y^s}\right)=O\left(\frac{1}{k^s}\right)+O\left(\frac{1}{y^s}\right) \tag{Su-72}$$

Su-A.3.2. *Formulas involving* $b_\square$. Calculations completely analogous to those for the triangular lattice yield

$$\sum_{n\le y} b_\square(n)n^{-s} = \frac{1}{1-s}L(1,\chi_{-4})\,y^{1-s} + O(y^{\frac{1}{2}-s})$$

for $s<0$, whereas for $0<s<\frac{1}{2}$ we get

$$\sum_{n\le y} b_\square(n)n^{-s} = \frac{L(1,\chi_{-4})}{1-s}\,y^{1-s} + O(y^{1/2-s}).$$

For $\frac{1}{2}<s<1$ we get

$$\sum_{n\le y} b_\square(n)n^{-s} = \frac{L(1,\chi_{-4})}{1-s}\,y^{1-s} + C(s) + O(y^{1/2-s}),$$

with

$$C(s) = L(s,\chi_{-4})\zeta(s) - \sum_{m=1}^{\infty}\frac{\chi_{-4}(m)}{m^s}\sum_{d=1}^{m}\frac{1}{d^s} + \sum_{m=1}^{\infty}\frac{1}{m^s}\sum_{d=m+1}^{\infty}\frac{\chi_{-4}(d)}{d^s} + L(2s,\chi_{-4}).$$

The sums in $C(s)$ are Dirichlet series that converge for $\mathrm{Re}(s)>\frac{1}{2}$, and are thus analytic for $\mathrm{Re}(s)>\frac{1}{2}$. They converge absolutely for $\mathrm{Re}(s)>1$, and a reordering of terms shows that the last three terms add up to zero for $\mathrm{Re}(s)>1$, and hence due to the analyticity also for $\mathrm{Re}(s)>\frac{1}{2}$. Hence $C(s)=L(s,\chi_{-4})\zeta(s)$ and thus

$$\sum_{n\le y}\frac{b_\square(n)}{n^s} = \frac{L(1,\chi_{-4})}{1-s}\,y^{1-s} + L(s,\chi_{-4})\zeta(s) + O(y^{1/2-s}).$$

For $s=\frac{1}{2}$ the situation is again a bit more tricky and we want to avoid logarithmic error terms. The only two difficult terms are

$$\sum_{m\le\sqrt{y}}\frac{\chi_{-4}(m)}{m^s}\sum_{d=1}^{m}\frac{1}{d^s} \qquad \text{and} \qquad \sum_{m\le\sqrt{y}}\frac{1}{m^s}\sum_{d=m+1}^{\infty}\frac{\chi_{-4}(d)}{d^s}$$

The first term

$$\begin{aligned}\sum_{m\le\sqrt{y}}\frac{\chi_{-4}(m)}{m^s}\sum_{d=1}^{m}\frac{1}{d^s} &= \sum_{k\le(\sqrt{y}-1)/4}\left(\left(\frac{1}{(4k+1)^s}-\frac{1}{(4k+3)^s}\right)\sum_{d=1}^{4k+1}\frac{1}{d^s}-\frac{1}{(4k+3)^{2s}}\right)\\ &\quad + O\left(\frac{1}{\sqrt{y}^s}\right)\sum_{d\le\sqrt{y}}\frac{1}{d^s}\\ &= \sum_{k\le(\sqrt{y}-1)/4}\left(\frac{1}{(4k+1)^s}\left(\frac{2s}{4k+1}+O\left(\frac{1}{(4k+1)^2}\right)\right)\left(\frac{(4k+1)^{1-s}}{1-s}+O(1)\right)\right.\\ &\quad \left. -\frac{1}{(4k+3)^{2s}}\right) + O(y^{1/2-s})\end{aligned}$$

$$= \left(\frac{s}{1-s} - 1\right) \sum_{k \le (\sqrt{y}-1)/4} \frac{1}{(4k+1)^{2s}}$$
$$+ \sum_{k \le (\sqrt{y}-1)/4} O\left(\frac{1}{(4k+1)^{s+1}}\right) + O(y^{1/2-s})$$

is seen to be bounded for $1 > s \ge \frac{1}{2}$ and so is the second

$$\begin{aligned}\sum_{m \le \sqrt{y}} \frac{1}{m^s} \sum_{d=m+1}^{\infty} \frac{\chi_{-4}(d)}{d^s} &= \sum_{0 \le k \le (\sqrt{y}-1)/4} \sum_{j=1}^{4} \frac{1}{(4k+j)^s} \sum_{d=4k+j+1}^{\infty} \frac{\chi_{-4}(d)}{d^s} + O(y^{-s}) \\ &= \sum_{0 \le k \le (\sqrt{y}-1)/4} \Bigg( \left(\frac{1}{(4k+1)^s} + \frac{1}{(4k+2)^s}\right) \frac{-1}{2(4k+3)^s} \\ &\quad + \left(\frac{1}{(4k+3)^s} + \frac{1}{(4k+4)^s}\right) \frac{1}{2(4k+5)^s} + O\left(\frac{1}{k^{1+2s}}\right)\Bigg) + O(y^{-s}) \\ &= \sum_{0 \le k \le (\sqrt{y}-1)/4} O\left(\frac{1}{k^{1+2s}}\right) + O(y^{-s})\end{aligned}$$

where we have made use of

$$\begin{aligned}\sum_{d=4k}^{\infty} \frac{\chi_{-4}(d)}{d^s} &= \sum_{d=4k+1}^{\infty} \frac{\chi_{-4}(d)}{d^s} \\ &= \sum_{\ell=k}^{\infty} \left(\frac{1}{(4\ell+1)^s} - \frac{1}{(4\ell+3)^s}\right) \\ &= \sum_{\ell=k}^{\infty} \frac{1}{(4\ell+1)^s} \left(\frac{2s}{4\ell+1} + O\left(\frac{1}{(4\ell+1)^2}\right)\right) \\ &= \frac{1}{2(4k+1)^s} + O\left(\frac{1}{k^{1+s}}\right)\end{aligned}$$

and

$$\begin{aligned}\sum_{d=4k+2}^{\infty} \frac{\chi_{-4}(d)}{d^s} = \sum_{d=4k+3}^{\infty} \frac{\chi_{-4}(d)}{d^s} &= -\sum_{\ell=k}^{\infty} \left(\frac{1}{(4\ell+3)^s} - \frac{1}{(4\ell+5)^s}\right) \\ &= -\frac{1}{2(4k+3)^s} + O\left(\frac{1}{k^{1+s}}\right).\end{aligned}$$

Hence

$$\sum_{n \le y} \frac{b_{\Box}(n)}{n^{1/2}} = 2L(1, \chi_{-4})\, y^{1/2} + O(1).$$

For $s = 1$ we get

$$\sum_{n \le y} \frac{b_{\Box}(n)}{n} = L(1, \chi_{-4}) \log(y) + C(1) + O(y^{-1/2} \log(y)),$$

with

$$\begin{aligned} C(1) &= L(1,\chi_{-4})\gamma - \sum_{m=1}^{\infty} \frac{\chi_{-4}(m)}{m}\left(\log(m) + \sum_{d=1}^{m}\frac{1}{d}\right) \\ &\quad + \sum_{m=1}^{\infty}\frac{1}{m}\sum_{d=m+1}^{\infty}\frac{\chi_{-4}(d)}{d} + L(2,\chi_{-4}) \\ &= L(1,\chi_{-4})\gamma - \sum_{m=1}^{\infty}\frac{\chi_{-4}(m)}{m}\log(m) = L(1,\chi_{-4})\gamma + L'(1,\chi_{-4}). \end{aligned}$$

by a similar reordering and analyticity argument as above.

For $s > 1$ we get

$$\sum_{n\le y}\frac{b_\square(n)}{n^s} = L(s,\chi_{-4})\zeta(s) + \frac{L(1,\chi_{-4})}{1-s}\,y^{1-s} + O(y^{-s/2}),$$

where we again have used the identity

$$\text{(Su-73)} \qquad -\sum_{m=1}^{\infty}\frac{\chi_{-4}(m)}{m^s}\sum_{d=1}^{m}\frac{1}{d^s} + \sum_{m=1}^{\infty}\frac{1}{m^s}\sum_{d=m+1}^{\infty}\frac{\chi_{-4}(d)}{d^s} + L(2s,\chi_{-4}) = 0.$$

Summarising we have

**Theorem Su-8.**

$$\text{(Su-74)} \qquad \sum_{n\le y} b_\square(n)n^{-s} = \begin{cases} \frac{L(1,\chi_{-4})}{1-s}\,y^{1-s} + O(y^{1/2-s}) & \textit{for } s<\frac{1}{2} \\ 2L(1,\chi_{-4})\,y^{1/2} + O(1) & \textit{for } s=\frac{1}{2} \\ \frac{L(1,\chi_{-4})}{1-s}\,y^{1-s} + L(s,\chi_{-4})\zeta(s) + O(y^{1/2-s}) & \textit{for } \frac{1}{2}<s<1 \\ L(1,\chi_{-4})\log(y) + C_\square(1) + O(y^{-1/2}\log(y)) & \textit{for } s=1 \\ L(s,\chi_{-4})\zeta(s) + \frac{L(1,\chi_{-4})}{1-s}\,y^{1-s} + O(y^{-s/2}) & \textit{for } s>1 \end{cases}$$

*where*

$$\text{(Su-75)} \qquad C_\square(1) = L(1,\chi_{-4})\gamma + L'(1,\chi_{-4}) \approx 0.6462454.$$

Note that we have the following formula (see [Su-2])

$$\text{(Su-76)} \qquad \frac{L'(1,\chi_{-4})}{L(1,\chi_{-4})} = \log\left(M(1,\sqrt{2})^2\frac{e^\gamma}{2}\right) = \log\left(\Gamma\left(\frac{3}{4}\right)^4\frac{e^\gamma}{\pi}\right),$$

where $M(x,y)$ is the arithmetic-geometric mean of $x$ and $y$.

Su-A.3.3. *Formulas for $w_\square$.* For $s > -1$ we have

$$\begin{aligned}
\sum_{n\le y} w_{\square,even}(n)n^s &= \sum_{p<\sqrt{y/2}} \sum_{p<q\le \min([p\sqrt{3}],[y/(2p)])} (2pq)^s \\
&= \sum_{p\le\sqrt{y/(2\sqrt{3})}} (2p)^s \sum_{p<q<p\sqrt{3}} q^s + \sum_{\sqrt{y/(2\sqrt{3})}<p<\sqrt{y/2}} (2p)^s \sum_{p<q\le y/(2p)} q^s \\
&= \sum_{p\le\sqrt{y/(2\sqrt{3})}} (2p)^s \left(\frac{1}{s+1}\, p^{1+s}(3^{(s+1)/2}-1) + O(p^s)\right) \\
&\quad + \sum_{\sqrt{y/(2\sqrt{3})}<p<\sqrt{y/2}} (2p)^s \left(\frac{1}{s+1}\left(\frac{y^{s+1}}{(2p)^{s+1}} - p^{s+1}\right) + O(p^s) + O\left(\frac{y^s}{p^s}\right)\right) \\
&= \frac{2^s(3^{(s+1)/2}-1)}{2(s+1)^2}\frac{y^{s+1}}{2^{s+1}3^{(s+1)/2}} + O(y^{s+\frac{1}{2}}) + O(1) \\
&\quad + \frac{y^{s+1}}{2(s+1)}\log\left(\frac{\sqrt{y/2}}{\sqrt{y/(2\sqrt{3})}}\right) - \frac{2^s}{2(s+1)^2}\left(\frac{y^{s+1}}{2^{s+1}} - \frac{y^{s+1}}{2^{s+1}3^{(s+1)/2}}\right) \\
&= \frac{\log(3)}{8(s+1)} y^{s+1} + O(y^{s+\frac{1}{2}}) + O(1).
\end{aligned}$$

Similarly (again for $s > -1$)

$$\begin{aligned}
\sum_{n\le y} w_{\square,odd}(n)n^s &= \sum_{k<(\sqrt{y}-1)/2} \sum_{k<\ell\le\min([\sqrt{3}k+(\sqrt{3}-1)/2],[y/(4k+2)-1/2])} (2k+1)^s(2\ell+1)^s \\
&= \sum_{k\le\sqrt{y}/(2\sqrt[4]{3})-1/2} (2k+1)^s \sum_{k<\ell<k\sqrt{3}+(\sqrt{3}-1)/2} (2\ell+1)^s \\
&\quad + \sum_{\sqrt{y}/(2\sqrt[4]{3})-1/2<k<(\sqrt{y}-1)/2} (2k+1)^s \sum_{k<\ell\le y/(4k+2)-1/2} (2\ell+1)^s \\
&= \sum_{k\le\sqrt{y}/(2\sqrt[4]{3})-1/2} (2k+1)^s \frac{1}{2(s+1)} \underbrace{\left(\left(2k\sqrt{3}+\sqrt{3}\right)^{s+1} - (2k+1)^{s+1}\right)}_{(3^{(s+1)/2}-1)(2k+1)^{s+1}+O(k^s)} \\
&\quad + \sum_{\sqrt{y}/(2\sqrt[4]{3})-1/2<k<(\sqrt{y}-1)/2} (2k+1)^s \times \\
&\quad \times \left(\frac{1}{2(s+1)}\left(\frac{y^{s+1}}{(2k+1)^{s+1}} - (2k+1)^{s+1}\right) + O(k^s) + O\left(\frac{y^s}{(2k+1)^s}\right)\right) \\
&= \frac{3^{(s+1)/2}-1}{8(s+1)^2}\frac{y^{s+1}}{3^{(s+1)/2}} + O(y^{s+\frac{1}{2}}) + O(1) \\
&\quad + \frac{y^{s+1}}{4(s+1)}\log\left(\frac{\sqrt{y}}{\sqrt{y}/\sqrt[4]{3}}\right) - \frac{1}{8(s+1)^2}\left(y^{s+1} - \frac{y^{s+1}}{3^{(s+1)/2}}\right)
\end{aligned}$$

$$= \frac{\log(3)}{16(s+1)} y^{s+1} + O(y^{s+\frac{1}{2}}) + O(1),$$

For $s = -1$ we get

$$\sum_{n \le y} \frac{w_{\square,even}(n)}{n} = \sum_{p < \sqrt{y/2}} \sum_{p < q \le \min([p\sqrt{3}],[y/(2p)])} \frac{1}{2pq}$$

$$= \sum_{p \le \sqrt{y/(2\sqrt{3})}} \frac{1}{2p} \sum_{p<q<p\sqrt{3}} \frac{1}{q} + \sum_{\sqrt{y/(2\sqrt{3})} < p < \sqrt{y/2}} \frac{1}{2p} \sum_{p < q \le y/(2p)} \frac{1}{q}$$

$$= \sum_{p \le \sqrt{y/(2\sqrt{3})}} \frac{1}{2p} \left( \frac{\log(3)}{2} + \underbrace{\sum_{p<q<p\sqrt{3}} \frac{1}{q} - \frac{\log(3)}{2}}_{O\left(\frac{1}{p}\right)} \right)$$

$$+ \sum_{\sqrt{y/(2\sqrt{3})} < p < \sqrt{y/2}} \frac{1}{2p} \left( \log\left(\frac{y}{2p^2}\right) + O\left(\frac{1}{p}\right) + O\left(\frac{p}{y}\right) \right)$$

$$= \frac{\log(3)}{4} \left( \log\left(\sqrt{\frac{y}{2\sqrt{3}}}\right) + \gamma + O(y^{-1/2}) \right)$$

$$+ \underbrace{\sum_{p=1}^{\infty} \frac{1}{2p} \left( \sum_{p<q<p\sqrt{3}} \frac{1}{q} - \frac{\log(3)}{2} \right)}_{=: c_4} + O(y^{-1/2})$$

$$+ \frac{\log(y) - \log(2)}{2} \log\left(\sqrt[4]{3}\right)$$

$$- \frac{1}{2} \left( \left( \log\left(\sqrt{\frac{y}{2}}\right) \right)^2 - \left( \log\left(\sqrt{\frac{y}{2\sqrt{3}}}\right) \right)^2 \right) + O(y^{-1/2} \log(y))$$

$$= \frac{\log(3)}{8} \log(y) + \frac{\log(3)}{4} \left( \gamma - \frac{1}{8}\log(3) - \frac{1}{2}\log(2) \right) + c_4 + O(y^{-1/2}\log(y)).$$

where we have made use of

$$\left( \log\left(\sqrt{\frac{y}{2}}\right) \right)^2 - \left( \log\left(\sqrt{\frac{y}{2\sqrt{3}}}\right) \right)^2 = \log\left(\sqrt[4]{3}\right) \log\left(\frac{y}{2\sqrt[4]{3}}\right)$$

$$= \frac{\log(3)}{4} \left( \log(y) - \frac{1}{4}\log(3) - \log(2) \right)$$

Similarly

$$\sum_{n \le y} \frac{w_{\square,odd}(n)}{n} = \sum_{k < (\sqrt{y}-1)/2} \sum_{k < \ell \le \min([\sqrt{3}k + (\sqrt{3}-1)/2],[y/(4k+2)-1/2])} \frac{1}{(2k+1)(2\ell+1)}$$

$$= \sum_{k \le \sqrt{y}/(2\sqrt[4]{3}) - 1/2} \frac{1}{2k+1} \sum_{k<\ell<k\sqrt{3}+(\sqrt{3}-1)/2} \frac{1}{2\ell+1}$$

$$
\begin{aligned}
&+\sum_{\sqrt{y}/(2\sqrt[4]{3})-1/2<k<(\sqrt{y}-1)/2} \frac{1}{2k+1} \sum_{k<\ell\le y/(4k+2)-1/2} \frac{1}{2\ell+1} \\
&= \sum_{k\le \sqrt{y}/(2\sqrt[4]{3})-1/2} \frac{1}{2k+1}\left(\frac{1}{4}\log(3) + \underbrace{\sum_{k<\ell<k\sqrt{3}+(\sqrt{3}-1)/2} \frac{1}{2\ell+1} - \frac{1}{4}\log(3)}_{O\left(\frac{1}{k}\right)}\right) \\
&\quad + \sum_{\sqrt{y}/(2\sqrt[4]{3})-1/2<k<(\sqrt{y}-1)/2} \frac{1}{2k+1}\left(\frac{1}{2}\log\left(\frac{y}{(2k+1)^2}\right) + O\left(\frac{1}{k}\right) + O\left(\frac{k}{y}\right)\right) \\
&= \frac{1}{4}\log(3)\left(\frac{1}{2}\log\left(\frac{\sqrt{y}}{\sqrt[4]{3}}\right) + \frac{1}{2}\gamma + \frac{1}{2}\log(2) - 1 + O(y^{-1/2})\right) \\
&\quad + \underbrace{\sum_{k=1}^{\infty} \frac{1}{2k+1}\left(\sum_{k<\ell<k\sqrt{3}+(\sqrt{3}-1)/2} \frac{1}{2\ell+1} - \frac{1}{4}\log(3)\right)}_{=:\, c_5 + \frac{1}{4}\log(3)} + O(y^{-1/2}) \\
&\quad + \frac{\log(y)}{4}\log\left(\sqrt[4]{3}\right) - \frac{1}{4}\left((\log(\sqrt{y}))^2 - \left(\log\left(\frac{\sqrt{y}}{\sqrt[4]{3}}\right)\right)^2\right) + O(y^{-1/2}\log(y)) \\
&= \frac{\log(3)}{16}\log(y) + \frac{\log(3)}{8}\left(\gamma - \frac{1}{8}\log(3) + \log(2)\right) + c_5 + O(y^{-1/2}\log(y))
\end{aligned}
$$

where we have made use of

$$
\begin{aligned}
(\log(\sqrt{y}))^2 - \left(\log\left(\frac{\sqrt{y}}{\sqrt[4]{3}}\right)\right)^2 &= \log\left(\sqrt[4]{3}\right)\log\left(\frac{y}{\sqrt[4]{3}}\right) \\
&= \frac{\log(3)}{4}\left(\log(y) - \frac{1}{4}\log(3)\right).
\end{aligned}
$$

Summarizing we have

**Theorem Su-9.** *The asymptotic formulas for $w_{\square,even}$ and $w_{\square,odd}$ read*

$$\sum_{n\le y} w_{\square,even}(n) n^s = \frac{\log(3)}{8(s+1)} y^{s+1} + O(y^{s+\frac{1}{2}}) + O(1), \tag{Su-77}$$

$$\sum_{n\le y} w_{\square,odd}(n) n^s = \frac{\log(3)}{16(s+1)} y^{s+1} + O(y^{s+\frac{1}{2}}) + O(1) \tag{Su-78}$$

*for $s > -1$. Furthermore*

$$\sum_{n\le y} \frac{w_{\square,even}(n)}{n} = \frac{\log(3)}{8}\log(y) + c_{even} + O(y^{-1/2}\log(y)), \tag{Su-79}$$

$$\sum_{n\le y}\frac{w_{\Box,odd}(n)}{n}=\frac{\log(3)}{16}\log(y)+c_{odd}+O(y^{-1/2}\log(y)), \tag{Su-80}$$

*where*

(Su-81)

$$c_{even}=\frac{\log(3)}{4}\left(\gamma-\frac{\log(3)}{8}-\frac{\log(2)}{2}\right)+\sum_{p=1}^{\infty}\frac{1}{2p}\left(\sum_{p<q<p\sqrt{3}}\frac{1}{q}-\frac{\log(3)}{2}\right)$$
$$\approx -0.3966993$$

(Su-82)

$$c_{odd}=\frac{\log(3)}{8}\left(\gamma-\frac{\log(3)}{8}+\log(2)\right)+\sum_{k=0}^{\infty}\frac{1}{2k+1}\left(\sum_{k<\ell<k\sqrt{3}+(\sqrt{3}-1)/2}\frac{1}{2\ell+1}-\frac{1}{4}\log(3)\right)$$
$$\approx -0.2083500$$

## References


[Su-1] T.M. Apostol, *Introduction to Analytic Number Theory*, Springer, New York (1976).

[Su-2] P. Moree, Chebyshev's bias for composite numbers with restricted prime divisors, *Math. Comp.*, **73** (2004), 425–449.



Fakultät für Mathematik, Universität Bielefeld, Box 100131, 33501 Bielefeld, Germany

*E-mail address*: `pzeiner@math.uni-bielefeld.de`
